# Supplementary material for: Actor-Critic Provably Finds Nash Equilibria of Linear-Quadratic Mean-Field Games
Source: arXiv:1910.07498 source file (2019-10-16)
Supplement: Supplementary file 1 [file appendix.tex]

%!TEX root =main.tex

\section{Auxiliary Algorithms and Analysis}

\subsection{Actor-Critic Algorithm For Minimizing $J_2(K,b)$}\label{sec:ac_lqrb}

In this section, given the fixed policy parameter $K$, we propose an actor-critic-type algorithm to find optimal $\hat b(K)$ which minimizes the cost function $J_2(K,b)$.

\begin{lemma}\label{lemma:convex_J2}
For any given parameter $K$, the cost function $J_2(K, b)$ is $\nu_K$-strongly convex in $b$, where $\nu_K$ is some positive number depending on $K$.  Also, the maximum singular value $\iota_K$ of the Hessian $\nabla^2_{bb} J_2(K, b)$ satisfies that $0<\iota_K\leq [1-\rho(A-BK)]^{-2} \cdot (  \|B\|_*^2\cdot \|K\|_*^2\cdot \|R\|_* + \|B\|_*^2\cdot \|Q\|_* )$. 
\end{lemma}
\begin{proof}
Please see \S\ref{proof:lemma:convex_J2}. 
\end{proof}

\begin{algorithm}[htpb]
    \caption{Actor-Critic Algorithm For Minimizing $J_2(K,b)$.}\label{algo:ac_lqrb}
    \begin{algorithmic}[1]
    \STATE{{\textbf{Input:}} Fixed first policy parameter $K$, initial second policy parameter $b_0$, stepsize $\gamma^0$, number of iterations $N^2$ and tolerance $\varepsilon > 0$. }
    \STATE{\textbf{Output}: The second optimal policy parameter $b$ and the estimated population mean $\hat \mu^x_{K, b}$. }
    \STATE{\textbf{Initialization}: $b\gets b_0$; }
    \FOR{ $n = 0, 1, 2, \ldots, N^2$}
        \STATE\textbf{Critic Update:} obtain estimators $\hat\Upsilon_K$, $\hat q_{K,b}$ and $\hat \mu^x_{K, b}$ of the matrix $\Upsilon_K$, the vector $q_{K,b}$ and mean $\mu^x_{K, b}$, via a policy gradient evaluation algorithm, for example, Algorithm \ref{algo:pg_eval}; 
        \STATE\textbf{Actor Update:} update the policy by
        \#\label{eq:update_policyb}
        b \gets b -  \gamma^0\cdot \bigl[\hat \Upsilon_K^{22}(-K\hat \mu_{K, b}^x + b) + \hat \Upsilon_{K}^{21}\hat \mu_{K,b}^x +\hat  q_{K,b}\bigr],
        \#
    \ENDFOR
    \RETURN the final second policy parameter $b$ and estimated population mean $\hat \mu^x_{K, b}$. 
    \end{algorithmic}
\end{algorithm}

\begin{theorem}[Convergence of Algorithm \ref{algo:ac_lqrb}]\label{thm:ac_b}
Let the initial policy $\pi_{K, b_0}$ be stable. For a sufficiently small $\varepsilon > 0$, in Algorithm \ref{algo:ac_lqr}, we set the stepsize such that $\gamma^0\leq 1 - \rho(A-BK)$, and the total number of iterations 
\$
N \geq C\cdot \nu_K^{-1}\cdot (\gamma^0)^{-1} \cdot \log\Bigl\{ 2\bigl[J_2(K, b_0) - J_2(K, b^K)\bigr]/\varepsilon \Bigr\},
\$ 
where $C$ is some positive absolute constant. 
Moreover, let $\{b_n\}_{n\in[N]}$ be the sequence of policy parameter pairs generated by the algorithm, and in the $n$-th iteration, we set the number of iterations $T^\mu_n$ and $T_n$ in Algorithm \ref{algo:pg_eval} such that 
\$
& T_n \geq \poly\bigl( \|K\|_\F, \|b_n\|_2, \|\mu\|_2, J_2(K, b_0) \bigr)\cdot \lambda_K^{-4}\cdot \nu_K^{-4}\cdot \bigl[1-\rho(A-BK)\bigr]^{-10}\cdot \varepsilon^{-5},\\
& T_n^\mu \geq \poly\bigl( \|K\|_\F, \|b_n\|_2, \|\mu\|_2, J_2(K, b_0) \bigr)\cdot \lambda_K^{-2}\cdot \nu_K^{-2}\cdot \bigl[1-\rho(A-BK)\bigr]^{-2}\cdot \varepsilon^{-2},
\$
where $\nu_K$ is specified in Lemma \ref{lemma:convex_J2}. 
Then with probability at least $1 - \varepsilon^{10}$, it holds that $J_2(K, b_N) - J_2(K, b^K) < \varepsilon$ and $\|b_N - b^K\|_2\leq \sqrt{2\varepsilon / \nu_K}$. 
\end{theorem}
\begin{proof}
Please see \S\ref{proof:thm:ac_b}. 
\end{proof}

\subsection{Primal-Dual Policy Gradient Evaluation Algorithm}\label{sec:pe_algo}

In the sequel, we derive the policy gradient evaluation algorithm, which is used in \textbf{Critic Update} in both Algorithm \ref{algo:ac_lqr} and Algorithm \ref{algo:ac_lqrb}, based on gradient temporal difference algorithm \citep{sutton2009fast}.  We proceed to evaluate the policy gradient for fixed policy $\pi = (K,b)$.  For notational convenience, we denote by 
\#\label{eq:def_feature}
\psi (x,u) = \begin{pmatrix}
\varphi(x,u)\\
x - \mu^x_{K,b}\\
u -  (-K\mu^x_{K,b} + b)\\
\end{pmatrix}
\#
the feature vector, where
\$
\varphi(x,u) = \svec\Biggl[
\begin{pmatrix}
x - \mu^x_{K,b}\\
u -  (-K\mu^x_{K,b} + b)
\end{pmatrix}
\begin{pmatrix}
x - \mu^x_{K,b}\\
u -  (-K\mu^x_{K,b} + b)
\end{pmatrix}^\top\Biggr]. 
\$
In order to write the quadratic state-action value function $Q_{K,b}(x,u)$ in a linear representation, we also denote by the vector
\#\label{eq:q1}
\alpha_{K,b} = \begin{pmatrix}
\svec(\Upsilon_K )\\
\Upsilon_K 
\begin{pmatrix}
\mu^x_{K,b}\\
-K\mu^x_{K,b} + b
\end{pmatrix} + \begin{pmatrix}
p_{K,b}\\
q_{K,b}
\end{pmatrix}
\end{pmatrix},
\#
where the matrix $\Upsilon_K$ is given in \eqref{eq:def_upsilon}. 
Note that according to the definition of $Q_{K,b}$ given in \eqref{eq:4b}, we can write $Q_{K,b}$ in the following form
\#\label{eq:q3}
Q_{K,b}(x,u) =  \psi(x,u)^\top \alpha_{K,b} + \beta_{K,b},
\#
where $\beta_{K,b}$ is a constant independent of $x$ and $u$. We also define the following matrix
\#\label{eq:q2}
\Theta_{K,b} = \EE_{\pi_{K,b}}\Bigl\{\psi(x,u)\bigl[ \psi(x,u) - \psi(x',u') \bigr] ^\top   \Bigr\},
\#
where $(x',u')$ is the state-action pair after $(x,u)$, and the expectation is taken following the policy $\pi_{K,b}$. Under the above notations, we establish the following proposition.

\begin{proposition}\label{prop:bellman_compact}
The following equation holds:
\#\label{eq:q8}
\begin{pmatrix}
1 & 0\\
\EE_{\pi_{K,b}}\bigl[ \psi(x,u) \bigr] & \Theta_{K,b}
\end{pmatrix}
\begin{pmatrix}
J(K,b)\\
\alpha_{K,b}
\end{pmatrix} = \begin{pmatrix}
J(K,b)\\
\EE_{\pi_{K,b}}\bigl[ c(x,u) \psi(x,u) \bigr]
\end{pmatrix},
\#
where the vector $\alpha_{K,b}$ is given in \eqref{eq:q1}, while the matrix $\Theta_{K,b}$ is given in \eqref{eq:q2}. 
\end{proposition} 
\begin{proof}
Please see \S\ref{proof:prop:bellman_compact}. 
\end{proof}

Motivated by Proposition \ref{prop:bellman_compact}, to obtain the parameter $\alpha_{K,b}$ of the value function, we proceed to solve the following linear system
\#\label{eq:linear_sys}
\tilde \Theta_{K,b} \cdot  \zeta
= \begin{pmatrix}
J(K,b)\\
\EE_{\pi_{K,b}}\bigl[ c(x,u) \psi(x,u) \bigr]
\end{pmatrix},
\#
where $\tilde \Theta_{K,b}$ is the matrix in the LHS of \eqref{eq:q8} and $\zeta = (\zeta_1, \zeta_2^\top)^\top$ is the vector of concern.    Note that in the above linear system \eqref{eq:linear_sys}, if the matrix $\Theta_{K,b}$ is invertible, then the whole linear system has unique solution $\zeta_{K,b} = (J(K,b), \alpha_{K,b}^\top)^\top$.    Fortunately, under mild requirement, the following proposition supports the invertibility of $\Theta_{K,b}$. 

\begin{proposition}\label{prop:invert_theta}
Under the above setting, if $\rho(A-BK) < 1$, then the matrix $\Theta_{K,b}$ is invertible, and its spectral norm is bounded by $4 ( 1 + \|K\|_\F^2 )^2\cdot \|\Phi^x_K\|_*^2$.  Moreover, the minimum singular value of the matrix $\tilde \Theta_{K,b}$ can be lower bounded by a positive constant $\lambda_K$, where $\lambda_K$ only depends on $\sigma$, $\sigma_{\min}(\Psi_\omega)$ and $\rho(A-BK)$. 
\end{proposition}
\begin{proof}
Please see \S\ref{proof:prop:invert_theta}. 
\end{proof}

To obtain the state-action value function, we only need to solve the linear system proposed in \eqref{eq:linear_sys}.  Instead of solving the linear system directly, we minimize the following loss function
\$
 \bigl[\zeta^1 - J(K,b)\bigr]^2 + \Bigl\| \EE_{\pi_{K,b}}\bigl[\psi(x,u)\bigr]  \zeta^1+ \Theta_{K,b} \zeta^2 -\EE_{\pi_{K,b}}\bigl[ c(x,u) \psi(x,u) \bigr] \Bigr\|_2^2. 
\$
Moreover, by Fenchel's duality, we can further convert the above minimization problem to the following min-max problem
\#\label{eq:minmax_pe}
\min_{\zeta\in\cV_\zeta}\max_{\xi\in\cV_\xi} F(\zeta, \xi)& = \Bigl\{  \EE_{\pi_{K,b}}\bigl[\psi(x,u)\bigr] \zeta^1+ \Theta_{K,b} \zeta^2 - \EE_{\pi_{K,b}}\bigl[ c(x,u) \psi(x,u) \bigr]\Bigr\}^\top \xi^2\notag\\
&\qquad  + \bigl[\zeta^1 - J(K,b)\bigr] \cdot \xi^1 - 1/2\cdot \|\xi\|_2^2 . 
\#
Here we restrict the primal variable $\zeta$ in some compact set $\cV_\zeta$ and the dual variable $\xi$ in some compact set $\cV_\xi$.  
By taking the gradient of the objective in \eqref{eq:minmax_pe} w.r.t. the primal variable $\zeta$ and the dual variable $\xi$, we obtain the follows
\$
& \nabla_{\zeta^1} F = \xi^1 + \EE_{\pi_{K,b}}\bigl[ \psi(x,u) \bigr]^\top \xi^2, \quad && \nabla_{\zeta^2} F = \Theta_{K,b}^\top \xi^2  , \\
&  \nabla_{\xi^1} F = \zeta^1 - J(K,b)-\xi^1, \qquad && \nabla_{\xi^2} F  = \EE_{\pi_{K,b}}\bigl[\psi(x,u)\bigr] \zeta^1+ \Theta_{K,b} \zeta^2  - \EE_{\pi_{K,b}}\bigl[ c(x,u) \psi(x,u) \bigr] - \xi^2. 
\$

Note that in the definition of the feature vector in \eqref{eq:def_feature}, we need the mean $\mu^x_{K,b}$ of the state to evaluate the feature. Therefore, prior to the policy evaluation, we need to estimate the mean, and formulate the estimated feature vector $\hat\psi(x,u)$ by replacing $\mu^x_{K,b}$ by $\hat\mu^x_{K,b}$ in the definition of $\psi(x,u)$ in \eqref{eq:def_feature}. Now, by stochastic gradient method, we propose the following policy gradient evaluation algorithm in Algorithm \ref{algo:pg_eval}.  In the follows, for notational convenience, we denote by $\hat\psi_t$ as the estimated feature $\hat\psi(x_t, u_t)$.

\begin{algorithm}[htpb]
    \caption{Primal-Dual Policy Gradient Evaluation Algorithm.}\label{algo:pg_eval}
    \begin{algorithmic}[1]
    \STATE{{\textbf{Input:}} Current policy $\pi = (K,b)$, number of iteration $T^\mu$, $T$ and stepsizes $\{\gamma_t\}_{t\in[T]}$. }
    \STATE{\textbf{Output}: Estimators $\hat\mu^x_{K,b}$ and $\hat \alpha_{K, b} $ of $\mu^x_{K,b}$ and $\alpha_{K, b}$ in \eqref{eq:q1}, respectively. Also, the estimators $\hat\Upsilon_K$, $\hat p_{K, b}$ and $\hat q_{K, b}$ of $\Upsilon_K$, $p_{K, b}$ and $q_{K, b}$ defined in \eqref{eq:def_upsilon}. }
    \STATE{Sample $x_0$ from the original population.}
    \FOR{ $t =  1, \ldots, T^\mu$}
        \STATE{Take action $u_{t-1}^\mu$ under the policy $\pi_{K,b}$ and generate the next state $x_{t}^\mu$.}
    \ENDFOR
    \STATE{Define the estimator of the mean as $\hat\mu^x_{K,b} = 1/T^\mu\cdot \sum_{t = 1}^{T^\mu} x_t^\mu$. }
    \STATE{Sample $x_0\sim\mathcal N(\mu^x_{K,b}, \Phi^x_K)$.}
    \FOR{ $t =  1, \ldots, T$}
        \STATE{Take action $u_{t-1}$ under the policy $\pi_{K,b}$, observe the cost $c_{t-1}$, and generate the next state $x_{t}$.}
        \STATE{Define the TD-error as 
        \#\label{eq:def_tderror}
        \delta_t = \zeta_{t-1}^1  + (\hat \psi_{t-1} - \hat\psi_t)^\top \zeta_{t-1}^2   - c_{t-1}.
        \#\vskip-10pt}
        \STATE{Update $\zeta^1$, $\zeta^2$, $\xi^1$ and $\xi^2$ as follows
        \#\label{eq:update_primal_dual}
        & \zeta_t^1 = \zeta_t^1 - \gamma_t\cdot (\xi_{t-1}^1 + \hat \psi_{t-1}^\top \xi_{t-1}^2), \qquad &&\zeta_t^2 = \zeta_t^2 - \gamma_t\cdot \hat \psi_{t-1}(\psi_{t-1} - \psi_t)^\top \xi_{t-1}^2, \notag  \\
        & \xi_{t}^1 = (1-\gamma_t)\cdot \xi_{t-1}^1 + \gamma_t \cdot (\zeta_{t-1}^1 -  c_{t-1}), \qquad &&\xi_{t}^2 = (1-\gamma_t)\cdot \xi_{t-1}^2 + \gamma_t \cdot\delta_t\cdot \hat\psi_{t-1}. 
        \#\vskip-10pt}
        \STATE{Project $\zeta_t$ and $\xi_t$ to the compact sets $\cV_\zeta$ and $\cV_\xi$, respectively. }
    \ENDFOR
    \STATE{Return $\hat\mu^x_{K,b}$ as the estimator of $\mu^x_{K,b}$.  Define $\hat\zeta^1 = (\sum_{t=1}^T \gamma_t)^{-1}\cdot(\sum_{t=1}^T \gamma_t \cdot \zeta_t^1)$ and $\hat\zeta^2 = (\sum_{t=1}^T \gamma_t)^{-1}\cdot(\sum_{t=1}^T \gamma_t\cdot \zeta_t^2)$. Then return 
    \$
    \hat J = \hat\zeta^1, \qquad \hat\alpha_{K, b} = \hat\zeta^2
    \$ 
    as the estimator of $J(K,b)$ and $\alpha_{K, b} $.    Denote by $\hat\alpha_{K, b}^1 =  (\hat\alpha_{K, b})_{1}^{(k+d+1)(k+d)/2}$ and $\hat\alpha_{K, b}^2 =  (\hat\alpha_{K, b})_{(k+d+1)(k+d)/2+1}^{(k+d+3)(k+d)/2}$, then return 
    \$
    \hat\Upsilon_K = \smat(\hat\alpha_{K, b}^1), \qquad\begin{pmatrix}\hat p_{K, b}\\ \hat q_{K, b}\end{pmatrix} = \hat\alpha_{K, b}^2 - \hat\Upsilon_{K}\begin{pmatrix}
    \hat\mu^x_{K,b}\\
    -K \hat\mu^x_{K,b} + b
    \end{pmatrix}
    \$
    as estimators of $\Upsilon_K$, $p_{K, b}$ and $q_{K, b}$.   }
    \end{algorithmic}
\end{algorithm}

Note that in the algorithm, actually we target on the empirical min-max problem:
\#\label{eq:minmax_pe_emp}
\min_{\zeta\in\cV_\zeta}\max_{\xi\in\cV_\xi} \hat F(\zeta, \xi)& = \Bigl\{  \EE_{\pi_{K,b}}\bigl[\hat \psi(x,u)\bigr] \zeta^1+ \hat \Theta_{K,b} \zeta^2 - \EE_{\pi_{K,b}}\bigl[ c(x,u) \hat \psi(x,u) \bigr]\Bigr\}^\top \xi^2\notag\\
&\qquad  + \bigl[\zeta^1 - J(K,b)\bigr] \cdot \xi^1 - 1/2\cdot \|\xi\|_2^2,
\#
where compared with the original min-max problem in \eqref{eq:minmax_pe},  the feature vector $\psi(x,u)$ is replaced by the estimated feature vector $\hat\psi(x,u)$. 

Note that the vector $\hat\zeta^2$ actually is an estimate of $\alpha_{K,b}$ in \eqref{eq:q1}, therefore, by taking its first $(k+d)(k+d+1)/2$ entries, we establish an estimate of $\Upsilon_K $.

\begin{assumption}\label{assum:proj}
Let $\pi_{K_0, b_0}$ be the initial policy in Algorithm \ref{algo:ac_lqr}. Assume that this initial policy is stable in the sense that $\rho(A-BK_0) < 1$. Consider the policy evaluation problem for the policy $\pi_{K,b}$, we assume that $J(K,b) \leq J(K_0, b_0) =: J_0$.  Moreover, the compact sets $\cV_\zeta$ and $\cV_\xi$ in \eqref{eq:minmax_pe} is defined as
\$
& \cV_\zeta = \Bigl\{ \zeta\colon 0\leq \zeta^1\leq J_0, \|\zeta^2\|_2 \leq M_{\zeta,1} + M_{\zeta,2}\cdot(1+ \|K\|_\F)\cdot \bigl[ 1-\rho(A-BK) \bigr]^{-1}  \Bigr\}, \\
& \cV_\xi = \Bigl\{ \xi\colon |\xi^1|\leq J_0, \|\xi^2\|_2\leq M_\xi\cdot \bigl(1+ \|K\|_\F^2 \bigr)^3 \cdot \bigl[ 1-\rho(A-BK) \bigr]^{-1} \Bigr\}. 
\$
Here $M_{\zeta,1}$, $M_{\zeta,2}$ and $M_\xi$ are constants independent of $K$ and $b$, which take the following forms
\$
&M_{\zeta,1} = \Bigl[ \bigl(\|Q\|_\F + \|R\|_\F\bigr) +  \bigl( \|A\|_\F^2 + \|B\|_\F^2 \bigr) \cdot \sqrt{d}\cdot  J_0/\sigma_{\min}(\Psi_\omega)  \Bigr]\\
&\qquad\qquad + \Bigl[ \bigl(\|Q\|_* + \|R\|_*\bigr) +  \bigl( \|A\|_* + \|B\|_* \bigr)^2 \cdot  J_0/\sigma_{\min}(\Psi_\omega)  \Bigr] \cdot \bigl[ J_0/\sigma_{\min}(Q) + J_0/\sigma_{\min}(R) \bigr]\\
&\qquad\qquad + \bigl( \|A\|_* + \|B\|_* \bigr) \cdot  J_0^2\cdot \sigma_{\min}^{-1}(\Psi_\omega)\cdot \sigma_{\min}^{-1}(Q)  ,\\
& M_{\zeta,2}  = \bigl( \|A\|_* + \|B\|_* \bigr) \cdot  (\kappa_Q + \kappa_R), \\ 
& M_\xi  = C\cdot (M_{\zeta,1} + M_{\zeta,2}) \cdot J_0^2/\sigma_{\min}^2(Q),
\$
where $C$ is an absolute constant, and $\kappa_Q$ and $\kappa_R$ are condition numbers of the matrices $Q$ and $R$. 
\end{assumption}

Under the above Assumption \ref{assum:proj}, we characterize the convergence of Algorithm \ref{algo:pg_eval} in the following theorem.

\begin{theorem}[Convergence of Policy Evaluation]\label{thm:pe}
Under Assumption \ref{assum:proj}, given the stepsize $\gamma_t = \gamma\cdot t^{-1/2}$ for some constant $\gamma>0$, then under Assumption \ref{assum:proj}, for any $\rho$ such that $\rho(A-BK) < \rho<1$, when the number of iterations $T^\mu$ and $T$ are sufficiently large, with probability at least $1-T^{-4} - (T^\mu)^{-6}$, the output $\hat\alpha_{K, b}$ satisfies that
\$
\|\hat\alpha_{K, b} - \alpha_{K, b}\|_2^2 \leq  \lambda_K^{-2}\cdot \poly\bigl( \|K\|_\F, \|b\|_2, \|\mu\|_2 \bigr)  \cdot  \biggl[  \frac{\log^6 T}{T^{1/2} \cdot (1-\rho)^{3}} +  \frac{\log T^\mu}{T^\mu}\biggr], 
\$
where $\lambda_K$ is specified in Proposition \ref{prop:invert_theta}.  Also, as a by-product, we have exactly the same bound for $\|\hat\Upsilon_K - \Upsilon_K\|_\F$, $\|\hat p_{K,b} - p_{K,b}\|_2$ and $\|\hat q_{K,b} - q_{K,b}\|_2$. 
\end{theorem}
\begin{proof}
Please see \S\ref{proof:thm:pe}. 
\end{proof}

\section{Proofs of Theorems}
\subsection{Proof of Theorem \ref{thm:pg}}\label{proof:thm:pg}
\begin{proof}
It can be shown that 
\#\label{eq:grad1}
\nabla_K \bigl[ \tr(P_K\Psi_\epsilon) \bigr] = 2\bigl[ (R+B^\top P_K B)K - B^\top P_K A \bigr]\Phi_K^x,
\#
also, we have
\#
&\nabla_K\bigl[ (\mu_{K,b}^x)^\top (Q+K^\top RK)\mu_{K,b}^x \bigr] = 2\bigl[ RK - B^\top(I-A+BK)^{-\top}(Q+K^\top RK) \bigr]\mu_{K,b}^x(\mu_{K,b}^x)^\top,\label{eq:grad2}\\
& \nabla_K(b^\top RK\mu_{K,b}^x) = \bigl[R-B^\top(I-A+BK)^{-\top}K^\top R\bigr]b(\mu_{K,b}^x)^\top. \label{eq:grad3}
\#
Combining the above equations, we obtain \eqref{eq:f3c} and \eqref{eq:f3a}. Moreover, \eqref{eq:f3b} is obtained simply by taking gradient w.r.t. $b$, combining the definition of $\mu_{K,b}^x$ in \eqref{eq:f2q} and the Lyapunov equation \eqref{eq:f2p}.  This concludes the theorem.
\end{proof}

\subsection{Proof of Theorem \ref{thm:pe}}\label{proof:thm:pe}
\begin{proof}
\textbf{Part 1.} We proceed to show that $(\zeta_{K,b}, 0)$ is a saddle point of the problem \eqref{eq:minmax_pe}. We first show that $\zeta_{K,b}\in\cV_\zeta$ and $\xi(\zeta)\in\cV_\xi$ for any $\zeta\in\cV_\zeta$, where $\xi(\zeta)$ is defined as $\xi(\zeta) = \argmax_\xi F(\zeta, \xi)$, by the following lemma.

\begin{lemma}\label{lemma:zeta_xi}
The vector $\zeta_{K,b} = (J(K,b), \alpha_{K,b}^\top)^\top\in\cV_\zeta$.  Moreover, for any $\zeta\in\cV_\zeta$, the vector $\xi(\zeta)$ defined above satisfies that $\xi(\zeta)\in\cV_\xi$. 
\end{lemma}
\begin{proof}
Please see \S\ref{proof:lemma:zeta_xi} for detailed proof. 
\end{proof}

Note that $\nabla_\zeta F(\zeta_{K,b}, 0) = 0$ and $\nabla_\xi F(\zeta_{K,b}, 0) = 0$, combining the above Lemma \ref{lemma:zeta_xi}, we know that $(\zeta_{K,b}, 0)$ is a saddle point of the function $F(\zeta, \xi)$ defined in the problem \eqref{eq:minmax_pe}.  This finishes the proof of our \textbf{Part 1}. 

\textbf{Part 2. }   We consider the primal-dual gap of the problem \eqref{eq:minmax_pe} defined as 
\#\label{eq:def_gap}
\gap (\hat \zeta, \hat \xi) = \max_{\xi\in\cV_\xi} F(\hat\zeta, \xi) - \min_{\zeta\in\cV_\zeta} F(\zeta, \hat\xi), 
\#
which indeed captures the performance of $(\hat\zeta, \hat\xi)$.  In the sequel, we proceed to relate \eqref{eq:def_gap} with the estimation error $\|\hat \alpha_{K, b} - \alpha_{K, b}\|_2$. 

First, note that for the estimator $\hat\zeta$ returned by Algorithm \ref{algo:pg_eval}, we have
\#\label{eq:gap1}
& \Bigl \|  \EE_{\pi_{K,b}}\bigl[\psi(x,u)\bigr] \hat\zeta^1+ \Theta_{K,b} \hat\zeta^2 - \EE_{\pi_{K,b}}\bigl[ c(x,u) \psi(x,u) \bigr] \Bigr\|^2_2   + \bigl |\hat\zeta^1 - J(K,b)\bigr |^2\notag\\
&\qquad = F\bigl[\hat\zeta, \xi(\hat\zeta) \bigr] = \max_{\xi\in\cV_\xi} F(\hat\zeta, \xi) = \gap (\hat\zeta, \hat\xi) + \min_{\zeta\in\cV_\zeta} F(\zeta, \hat\xi),
\#
where the second line comes from \eqref{eq:expl_xi} and the definition of $\xi(\zeta)$ in \textbf{Part 1}.  Moreover, note that for any $\xi\in\cV_\xi$, the follows hold:
\#\label{eq:gap2}
&\min_{\zeta\in\cV_\zeta} F(\zeta, \xi) \leq \min_{\zeta\in\cV_\zeta} \max_{\xi\in\cV_\xi} F(\zeta, \xi) = \min_{\zeta\in\cV_\zeta} F\bigl[ \zeta, \xi(\zeta) \bigr]\notag\\
& \qquad = \frac{1}{2}\cdot  \min_{\zeta\in\cV_\zeta}  \biggl\{   \Bigl \|  \EE_{\pi_{K,b}}\bigl[\psi(x,u)\bigr] \zeta^1+ \Theta_{K,b} \zeta^2 - \EE_{\pi_{K,b}}\bigl[ c(x,u) \psi(x,u) \bigr] \Bigr\|^2_2   + \bigl |\zeta^1 - J(K,b)\bigr |^2\biggr\}\notag\\
&\qquad = 0, 
\#
where the first line comes from the definition of $\xi(\zeta)$ in \textbf{Part 1}, the second line comes from \eqref{eq:expl_xi}, while the last equality holds by taking $\zeta = \alpha_{K, b}\in\cV_\zeta$.  
Further, we can establish a lower for the LHS of \eqref{eq:gap1} as follows
\#\label{eq:gap3}
& \Bigl \|  \EE_{\pi_{K,b}}\bigl[\psi(x,u)\bigr] \hat\zeta^1+ \Theta_{K,b} \hat\zeta^2 - \EE_{\pi_{K,b}}\bigl[ c(x,u) \psi(x,u) \bigr] \Bigr\|^2_2   + \bigl |\hat\zeta^1 - J(K,b)\bigr |^2\notag\\
&\qquad =\bigl \| \tilde \Theta_{K, b} (\hat\zeta - \zeta_{K, b})\bigr \|_2^2 \geq \lambda_K^2 \cdot \| \hat\zeta - \zeta_{K, b} \|_2^2 \geq  \lambda_K^2 \cdot \| \hat\alpha_{K, b} - \alpha_{K, b} \|_2^2,
\#
where the matrix $\tilde\Theta_{K, b}$ is given in \eqref{eq:linear_sys} and the scalar $\lambda_K$ is specified in Proposition \ref{prop:invert_theta}.  Combining \eqref{eq:gap1}, \eqref{eq:gap2} and \eqref{eq:gap3}, we obtain the relation between $\gap (\hat \zeta, \hat \xi)$ and $\|\hat \alpha_{K, b} - \alpha_{K, b}\|_2$:
\#\label{eq:gap_error}
\|\hat \alpha_{K, b} - \alpha_{K, b}\|_2^2 \leq \lambda_K^{-2} \cdot \gap(\hat\zeta, \hat\xi). 
\#

\textbf{Part 3. } We now proceed to upper bound the primal-dual gap $\gap(\hat\zeta, \hat\xi)$, then by \eqref{eq:gap_error} in \textbf{Part 2}, we establish the upper bound of the estimation error $\|\hat \alpha_{K, b} - \alpha_{K, b}\|_2$. Note that since the state $x$ and action $u$ actually follow Gaussian distributions, therefore, they are unbounded.    First we utilize Hansen-Wright inequality (Lemma \ref{lemma:hwineq}) to pick up an event where these two random variables are bounded. Before pick up such an event, the following Lemma \ref{lemma:dist_hat_muz} characterize the distribution of $\hat \mu_z = 1/T^\mu\cdot \sum_{t = 1}^{T^\mu} z_t^\mu$, where $z_t^\mu = [(x_t^\mu)^\top, (u_t^\mu)^\top]^\top$ is the concatenation of the state $x_t^\mu$ and the action $u_t^\mu$. 

\begin{lemma}\label{lemma:dist_hat_muz}
The running average $\hat \mu_z = 1/T^\mu\cdot \sum_{t = 1}^{T^\mu} z_t^\mu$, where $z_t^\mu = [(x_t^\mu)^\top, (u_t^\mu)^\top]^\top$, satisfies that
\$
\hat \mu_z\sim\mathcal N\biggl(\mu_z + \frac{1}{T^\mu}\mu_{T^\mu}, ~\frac{1}{T^\mu} \tilde \Sigma_{T^\mu} \biggr),
\$
where $\mu_{T^\mu}$ and $\tilde \Sigma_{T^\mu}$ are bounded in the sense that there exist absolute constant $M_\mu$ and $M_\Sigma$ such that $\|\mu_{T^\mu}\|_2\leq M_\mu\cdot \|\mu_z\|_2$ and $\|\tilde \Sigma_{T^\mu}\|_*\leq M_\Sigma\cdot \|\Sigma_z\|_*$, where $\Sigma_z$ is given in \eqref{eq:sigma_z_factor}. 
\end{lemma}
\begin{proof}
{\red easy proof}
\end{proof}

Now, note that the random variable $z-\hat\mu_z + 1/T^\mu\cdot \mu_{T^\mu} \sim\mathcal N(0,\Sigma_z + 1/T^\mu\cdot \tilde \Sigma_{T^\mu})$, by Lemma \ref{lemma:hwineq}, there exists an absolute constant $C_0>0$ such that 
\$
\PP\Bigl[   \bigl |  \| z-\mu_z + 1/T^\mu\cdot \mu_{T^\mu}  \|_2^2 - \tr(\tilde \Sigma_z)    \bigr|   >   \tau    \Bigr]  \leq  2\cdot  \exp\Bigl[ -C_0\cdot \min\bigl(  \tau^2 \|\tilde \Sigma_z\|_\F^{-2}, ~\tau\|\tilde \Sigma_z\|_*^{-1}  \bigr) \Bigr],
\$
where for notational convenience, we write $\tilde \Sigma_z = \Sigma_z + 1/T^\mu\tilde \Sigma_{T^\mu}$. 　
By taking $\tau = C_1\cdot \log T\cdot \|\tilde \Sigma_z\|_*$ for some sufficiently large absolute constant $C_1$, the above inequality takes the form
\#\label{eq:prob1}
\PP\Bigl[   \bigl |  \| z-\mu_z + 1/T^\mu\cdot \mu_{T^\mu}  \|_2^2 - \tr(\tilde \Sigma_z)    \bigr|   >   C_1\cdot \log T\cdot \|\tilde \Sigma_z\|_*    \Bigr]  \leq T^{-6}.
\#
We define the following event for any $t\in[T]$: 
\#\label{eq:def_event}
\cE_{t,1} = \Bigl\{   \bigl |  \| z_t -\mu_z + 1/T^\mu\cdot \mu_{T^\mu}  \|_2^2 - \tr(\tilde \Sigma_z)    \bigr|   \leq    C_1\cdot \log T\cdot \|\tilde \Sigma_z\|_*   \Bigr\}.
\#
Then by \eqref{eq:prob1}, we know that $\PP(\cE_{t,1}) \geq 1- T^{-6}$ for any $t\in[T]$. Also, we define $\cE_1 = \cap_{t\in[T]}\cE_{t,1}$, then we know that $\PP(\cE_1)\geq 1 - T^{-5}$ by union bound.   Also, by the definition of $\cE_1$, conditioning on the event $\cE_1$, it holds that
\#\label{eq:bound_z}
\max_{t\in[T]} \|z_t - \mu_z\|_2^2 &  \leq     C_1\cdot \log T\cdot \|\tilde \Sigma_z\|_* + \tr(\tilde \Sigma_z) + \| 1/T^\mu\cdot \mu_{T^\mu}\|_2^2\notag \\
&\leq   2 C_1\cdot \bigl[1 + M_\Sigma/(T^\mu)^2 \bigr] \cdot \log T\cdot \| \Sigma_z\|_*  + M_\mu / (T^\mu)^2\cdot \|\mu_z\|_2^2\notag \\
& \leq C_2\cdot \log T\cdot \bigl(1+\|K\|_\F^2\bigr)\cdot \|\Phi_K^x\|_* +   C_3\cdot  \bigl(\|b\|_2^2 + \|\mu\|_2^2 \bigr) \cdot (1-\rho)^{-2} \cdot  (T^\mu)^{-2}\notag\\
& \leq  2C_2\cdot \log T\cdot \bigl(1+\|K\|_\F^2\bigr)\cdot \|\Phi_K^x\|_*
\#
for sufficiently large $T^\mu$. 
Here $C_2$ and $C_3$ are positive absolute constants.   Moreover, we define the following event
\#\label{eq:def_event2}
\cE_2 = \bigl\{    \| \hat\mu_z -\mu_z + 1/T^\mu\cdot \mu_{T^\mu}  \|_2     \leq    C_1\bigr\}. 
\#
Then by Lemma \ref{lemma:dist_hat_muz}, we know that $\PP(\cE_2) \geq 1 - (T^\mu)^{-6}$.  We define the event $\cE$ as the intersection of the event $\cE_1$ and $\cE_2$, then by union bound, it is easy to show that $\PP(\cE)\geq 1- T^{-5} - (T^\mu)^{-6}$. 

Now, we define the truncated feature vector $\tilde \psi(x,u)$ conditioning on the proposed event $\cE$ as $\tilde \psi(x,u) = \hat \psi(x,u)\ind_{\cE}$, and also the truncated objective function as follow
\#\label{eq:trun_obj}
\tilde F(\zeta, \xi) =  \Bigl\{  \EE ( \tilde \psi ) \zeta^1+ \EE \bigl[ (\tilde \psi - \tilde \psi') \tilde \psi^\top \bigr] \zeta^2 - \EE ( \tilde c \tilde \psi )\Bigr\}^\top \xi^2  + \bigl[\zeta^1 - \EE (\tilde c)\bigr] \cdot \xi^1 - 1/2\cdot \|\xi\|_2^2,
\#
where the expectation is taken over the trajectory generated by the policy $\pi_{K, b}$, we write $\tilde \psi = \tilde \psi(x,u)$ to simplify the notations, and the function $\tilde c(x,u)$ is the truncated cost, which is defined as $\tilde c(x,u) = c(x,u)\ind_{\cE}$. The following lemma establishes the upper bound of $|F(\zeta, \xi) - \tilde  F(\zeta, \xi)|$, where $F(\zeta, \xi)$ and $\tilde F(\zeta, \xi)$ are given in \eqref{eq:minmax_pe} and \eqref{eq:trun_obj} respectively. 

\begin{lemma}\label{lemma:bound_tilde_F}
Given $F(\zeta, \xi)$ and $\tilde F(\zeta, \xi)$ in \eqref{eq:minmax_pe} and \eqref{eq:trun_obj}, it holds that
\$
|F(\zeta, \xi) - \tilde F(\zeta, \xi)|  \leq  \frac{1}{2T} + \frac{\log T^\mu}{T^\mu}\cdot \poly\bigl( \|K\|_\F, \|b\|_2, \|\mu\|_2 \bigr),
\$
with probability at least $1-(T^\mu)^{-6}$. 
\end{lemma}
\begin{proof}
Please see \S\ref{proof:lemma:bound_tilde_F}. 
\end{proof}

By the above Lemma \ref{lemma:bound_tilde_F}, we know that with probability at least $1-(T^\mu)^{-6}$, it holds that
\#\label{eq:gap_tilde_bound}
\Biggl| \gap(\hat \zeta, \hat \xi) - \biggl[  \max_{\xi\in\cV_\xi} \tilde F(\hat\zeta, \xi) - \min_{\zeta\in\cV_\zeta} \tilde F(\zeta, \hat\xi)   \biggr] \Biggr| \leq \frac{1}{T} + \frac{\log T^\mu}{T^\mu}\cdot \poly\bigl( \|K\|_\F, \|b\|_2, \|\mu\|_2 \bigr).
\#
Therefore, to obtain the bound of $\gap(\zeta, \xi)$, we only need to bound the term $\max_{\xi\in\cV_\xi} \tilde F(\hat\zeta, \xi) - \min_{\zeta\in\cV_\zeta} \tilde F(\zeta, \hat\xi)$ in \eqref{eq:gap_tilde_bound}.    We first use the following lemma to characterize the dependency of the trajectories generated by \eqref{eq:slqr}. 

\begin{lemma}\label{lemma:mixing}
Consider a linear dynamical system $x_{t+1} = D x_t + d + \epsilon_t$, where $\{x_t\}_{t\geq 0}\subset \RR^m$, the matrix $D\in\RR^{m\times m}$ satisfying $\rho(D) < 1$, the vector $d\in\RR^m$, and $\epsilon_t\sim\mathcal N(0, \Sigma)$ is the Gaussians. We denote by $\varpi_t$ the marginal distribution of $x_t$ for each $t\geq0$. Besides, it is easy to verify that the stationary distribution of this Markov chain is a Gaussian distribution $\mathcal N((I-D)^{-1}d, \Sigma_\infty)$, where $\Sigma_\infty$ is the covariance matrix of this distribution. We define the $\beta$-mixing coefficients for each $n\geq 1$ as follows
\$
\beta(n) = \sup_{t\geq 0} \EE_{x\sim \varpi_t} \Bigl[   \bigl\| \PP_{x_n}(\cdot\given x_0 = x) - \PP_{\mathcal N((I-D)^{-1}d, \Sigma_\infty)} (\cdot )  \bigr\|_\TV   \Bigr].
\$
Then, for any $\rho\in(\rho(D), 1)$, the mixing coefficients satisfy that 
\$
\beta(n) \leq C_{\rho, D}  \cdot \bigl[ \tr(\Sigma_\infty) + m\cdot (1-\rho)^{-2} \bigr]^{1/2}\cdot \rho^n,
\$
where the scalar $C_{\rho, D, d}$ is a constant which only depends on $\rho$, $D$ and $d$.   We say that the sequence $\{x_t\}_{t\geq 0}$ is $\beta$-mixing with parameter $\rho$. 
\end{lemma}
\begin{proof}
Please see \cite{tu2017least}.
\end{proof}

Note that under the dynamical system \eqref{eq:slqr}, the generated sequence $\{x_t\}_{t\geq 0}$ actually follows the dynamics proposed in \eqref{eq:f1}, where the matrix $A-BK$ satisfies that $\rho(A-BK) < 1$. Therefore, according to Lemma \ref{lemma:mixing}, we know that the sequence $\{z_t = (x_t^\top, u_t^\top)^\top\}_{t\geq 0}$ is $\beta$-mixing with parameter $\rho\in(\rho(A-BK),1)$.   Now the following lemma helps us to establish the primal-dual gap for a convex-concave problem.

\begin{lemma}\label{lemma:primal_dual_gap}
Let $\cX$ and $\cY$ be two compact and convex sets such that $\|x-x'\|_2 \leq M$ and $\|y-y'\|_2 \leq M$ for any $x,x'\in\cX$ and $y,y'\in\cY$. We consider solving the following problem
\$
\min_{x\in\cX}\max_{y\in\cY} F(x,y) = \EE_{\epsilon\sim \varpi_\epsilon} \bigl[ G(x,y;\epsilon) \bigr],
\$ 
where the objective function $F(x,y)$ is convex in $x$ and concave in $y$. In addition, we assume that the distribution $\varpi_\epsilon$ is the stationary distribution induced by a Markov chain $\{\epsilon_t\}_{t\geq 0}$, which is $\beta$-mixing with $\beta(n) \leq C_\epsilon\cdot \rho^n$, where $C_\epsilon$ is a constant. Moreover, we assume that it holds almost surely that $G(x,y;\epsilon)$ is $L_0$-Lipschitz in both $x$ and $y$, the gradient $\nabla_x G(x,y;\epsilon)$ is $L_1$-Lipschitz in $x$ for any $y\in\cY$, the gradient $\nabla_y G(x,y;\epsilon)$ is $L_1$-Lipschitz in $y$ for any $x\in\cX$, where $C_\epsilon, L_1, L_2 > 1$. Each step of our gradient-based method takes the following form:
\$
x_{t+1} = \Gamma_{\cX} \bigl[ x_{t} - \gamma_{t+1} \cdot \nabla_x G(x_{t}, y_{t}; \epsilon_t)\bigr], \qquad y_{t+1} = \Gamma_{\cY} \bigl[ y_{t} - \gamma_{t+1} \cdot \nabla_y G(x_{t}, y_{t}; \epsilon_t)\bigr],
\$
where the operators $\Gamma_\cX$ and $\Gamma_\cY$ projects the variables back to $\cX$ and $\cY$, respectively, and the stepsizes take the form $\gamma_t = \gamma/\sqrt{t}$ for some constant $\gamma > 0$. Moreover, let $\hat x = (\sum_{t = 1}^T \gamma_t)^{-1} (\sum_{t = 1}^T \gamma_t x_t)$ and $\hat y = (\sum_{t = 1}^T \gamma_t)^{-1} (\sum_{t = 1}^T \gamma_t y_t)$ be the final output of the gradient method after $T$ iterations, then there exists an absolute constant $C>0$, such that for any $\delta\in(0,1)$, the primal-dual gap to the minimax optimization problem satisfies that
\$
\max_{x\in\cX} F(\hat x, y) - \min_{y\in\cY} F(x, \hat y) \leq \frac{C\cdot (M^2 + L_0^2 + L_0L_1 D)}{\log(1/\rho)} \cdot \frac{\log^2 T + \log(1/\delta)}{\sqrt{T}} + \frac{C\cdot C_\epsilon L_0 M}{T}
\$
with probability at least $1-\delta$. 
\end{lemma}
\begin{proof}
This theorem is a generalization of Theorem 1 in \citep{wang2017finite} 
\end{proof}

To utilize the above Lemma \ref{lemma:primal_dual_gap}, we define the function $G(\zeta, \xi; \tilde \psi, \tilde \psi')$ as
\$
G(\zeta, \xi; \tilde \psi, \tilde \psi') = \Bigl[  \tilde \psi  \zeta^1+  (\tilde \psi - \tilde \psi') \tilde \psi^\top  \zeta^2 -  \tilde c \tilde \psi \Bigr]^\top \xi^2  + (\zeta^1 -  \tilde c ) \cdot \xi^1 - 1/2\cdot \|\xi\|_2^2,
\$
whose gradient takes the form
\$
\nabla_\zeta G(\zeta, \xi; \tilde \psi, \tilde \psi') = \begin{pmatrix} 
\tilde \psi^\top \xi^2 + \xi^1\\
\tilde \psi (\tilde \psi - \tilde \psi')^\top \xi^2
\end{pmatrix}, \qquad
\nabla_\xi G(\zeta, \xi; \tilde \psi, \tilde \psi') = \begin{pmatrix} 
\zeta^1 - \tilde c - \xi^1\\
\tilde \psi  \zeta^1+  (\tilde \psi - \tilde \psi') \tilde \psi^\top  \zeta^2 -  \tilde c \tilde \psi - \xi^2
\end{pmatrix}.
\$
By calculations and Lemma \ref{lemma:zeta_xi}, we know that
\#\label{eq:grad_bound}
& \bigl\|\nabla_\zeta G(\zeta, \xi; \tilde \psi, \tilde \psi')  \bigr\|_2 \leq  \poly \bigl(  \|K\|_\F  \bigr)\cdot \log^2 T\cdot (1-\rho)^{-1}, \notag\\
& \bigl\|\nabla_\xi G(\zeta, \xi; \tilde \psi, \tilde \psi')  \bigr\|_2 \leq  \poly \bigl(  \|K\|_\F, \|\mu\|_2  \bigr)\cdot \log^2 T \cdot (1-\rho)^{-1}.
\#
And also, the Hessian takes the form
\$
\nabla^2_{\zeta\zeta} G(\zeta, \xi; \tilde \psi, \tilde \psi') = 0, \qquad \nabla^2_{\xi\xi} G(\zeta, \xi; \tilde \psi, \tilde \psi') = -I,
\$
which gives that
\#\label{eq:hess_bound}
\bigl\|\nabla^2_{\zeta\zeta} G(\zeta, \xi; \tilde \psi, \tilde \psi')\bigr\|_2 = 0, \qquad \bigl\|\nabla^2_{\xi\xi} G(\zeta, \xi; \tilde \psi, \tilde \psi')\bigr\|_2 = 1. 
\#
Now, combining \eqref{eq:bound_z}, \eqref{eq:grad_bound}, \eqref{eq:hess_bound} and Lemma \ref{lemma:primal_dual_gap}, we know that 
\$
\max_{\xi\in\cV_\xi} \tilde F(\hat\zeta, \xi) - \min_{\zeta\in\cV_\zeta} \tilde F(\zeta, \hat\xi) \leq \frac{\poly \bigl( \|K\|_\F, \|\mu\|_2  \bigr)\cdot \log^6 T}{(1-\rho)^{3}\cdot \sqrt{T}}
\$
holds with probability at least $1 - T^{-5}$.  Furthermore, combining \eqref{eq:gap_error} and  \eqref{eq:gap_tilde_bound}, we conclude the theorem.  
\end{proof}

\subsection{Proof of Theorem \ref{thm:ac_b}}\label{proof:thm:ac_b}
\begin{proof}  
Note that our proposed algorithm aims to minimize $J_2(K,b)$ for a fixed $K$; therefore, we write $J_2(b;K) = J_2(K,b)$ by treating $K$ as a parameter of the function $J_2$. 
We proceed our proof by first showing the fact that $J_2(b;K)$ is strongly convex, and then by using this fact to show the convergence of Algorithm \ref{algo:ac_lqrb} combining the convergence result of policy evaluation in Theorem \ref{thm:pe}. 

First, by Lemma \ref{lemma:convex_J2}, we know that $J_2(b;K)$ is strongly convex in $b$ and has Lipschitz gradient.

We now proceed to show the convergence of Algorithm \ref{algo:ac_lqrb}. First, we use mathematical induction to show that the sequence $\{ J_2(b_n;K) \}_{n\geq 0}$ is non-increasing with large probability, as long as $J_2(b_n;K) - J_2(b^K;K)\geq \varepsilon$. Suppose that $J_2(b_n;K)\leq J_2(b_{n-1};K)\leq  \cdots \leq J_2(b_0;K)$ (note that this holds for $n=0$).
  Recall that according to Algorithm \ref{algo:ac_lqrb}, the policy parameter $K$ is updated through the follows
\#\label{eq:ac_update_bn}
b_{n+1} = b_n -  \gamma^0\cdot \hat\nabla J_2(b_n; K),
\#
where $\hat\nabla J_2(b_n; K) = \hat \Upsilon_K^{22}(-K\hat \mu_{K, b_n}^x + b_n) + \hat \Upsilon_{K}^{21}\hat \mu_{K,b_n}^x +\hat  q_{K,b_n}$ is the approximate gradient at $b_n$, and $\hat \Upsilon_{K}$ is the output of Algorithm \ref{algo:pg_eval}.  We also define $\tilde b_{n+1}$ as an exact update: 
\#\label{eq:tilde_update_bn}
\tilde b_{n+1} = b_n -  \gamma^0\cdot \nabla J_2(b_n; K),
\#
where $\nabla J_2(b_n; K) =  \Upsilon_K^{22}(-K \mu_{K, b_n}^x + b_n) +  \Upsilon_{K}^{21} \mu_{K,b_n}^x +  q_{K,b_n}$ is the exact gradient at $b_k$, and $\Upsilon_{K}$ and $q_{K,b_n}$ are given in \eqref{eq:def_upsilon}.    We proceed to bound $J_2(b_{n+1}; K) - J_2(b^K; K)$ in the sequel, where $b^K = \argmin_{b} J_2(b; K)$.   

Note that by the convexity of $J_2(b;K)$ in Lemma \ref{lemma:convex_J2},  we have
\#\label{eq:diff_tildeb_b1}
& J_2(\tilde b_{n+1}; K) - J_2(b_n; K) \leq -\gamma^0\cdot \bigl\| \nabla J_2(b_n; K)\bigr\|_2^2 \leq -2\nu_K\cdot \gamma^0\cdot \bigl[ J_2(b_n; K) - J_2(b^K; K) \bigr].
\#
This also implies that $J_2(\tilde b_{n+1}) < J_2(b_n; K)$.  Now, we only need to establish the error bound $|J_2(\tilde b_{n+1}; K) - J_2( b_{n+1}; K)|$.  
The following lemma quantifies the above error bound $ \bigl|J_2(b_{n+1}; K) - J_2(\tilde b_{n+1}; K)\bigr|$ towards $0$ with a high probability. 

\begin{lemma}\label{lemma:bound_tilde_J_2}
Assume that $J_2(b_n; K) \leq J_2(b_0; K)$.  Under the conditions stated in Theorem \ref{thm:ac_b}, with probability at least $1-\varepsilon^{10}$, we have
\#\label{eq:lemma_bound_tilde}
\bigl|J_2(b_{n+1}; K) - J_2(\tilde b_{n+1}; K)\bigr|  \leq  \nu_K\cdot\gamma^0\cdot \varepsilon,
\#
where $\hat \nabla J_2(b_n; K)$ is the approximate gradient given in \eqref{eq:ac_update_bn}, while $\nabla J_2(b_n; K)$ is the exact gradient given in \eqref{eq:tilde_update_bn}.
\end{lemma}
\begin{proof}
Please see \S\ref{proof:lemma:bound_tilde_J_2}. 
\end{proof}

Now, by applying the above Lemma \ref{lemma:bound_tilde_J_2}, we know that  if $J_2(b_n; K) - J_2(b^K; K) \geq \varepsilon$, combining \eqref{eq:diff_tildeb_b1}, it holds with probability at least $1-\varepsilon^{10}$ that
\$
J_2(b_{n+1}; K) - J_2(b_{n}; K) \leq - \nu_K\cdot \gamma^0\cdot  \varepsilon < 0. 
\$
By this, we finish the mathematical induction that $\{ J_2(b_n; K) \}_{n\geq 0}$ is non-increasing with large probability, as long as $J_2(b_n; K) - J_2(b^K; K)\geq \varepsilon$.  

Also, when $J_2(b_n; K) - J_2(b^K; K)\geq \varepsilon$,  by \eqref{eq:diff_tildeb_b1} and \eqref{eq:lemma_bound_tilde}, with probability at least $1-\varepsilon^{10}$, it holds that
\$
J_2(b_{n+1}; K) - J_2(b^K; K) \leq (1-\nu_K\cdot \gamma^0)\cdot  \bigl[ J_2(b_{n}; K) - J_2(b^K; K)\bigr],
\$ 
which proves the linear convergence rate of our proposed Algorithm \ref{algo:ac_lqrb}. Moreover, combining the fact that $J_2(\cdot; K)$ is strongly convex as shown in Lemma \ref{lemma:convex_J2}, we concludes the theorem. 
\end{proof}

\subsection{Proof of Theorem \ref{thm:ac}}\label{proof:thm:ac}
\begin{proof}  
Note that by Algorithm \ref{algo:ac_lqr}, the policy parameter $b_n$ attains its optimal $b_n = b^{K_n}$ given $K_n$ at $n$-th iteration. 
Recall that in Proposition \ref{prop:cost_form}, we decompose $J(K, b)$ into $J(K,b) = J_1(K) + J_2(K,b)+ \sigma^2 \cdot \tr(R) + \mu^\top \overline Q \mu$, where the term $J_2(K,b)$ is a constant independent of $K$ by Proposition \ref{prop:J2} if we take $b$ to be the optimal parameter $b^K$. From this fact, we can see that
\$
J(K_N, b_N) - J(K^*, b^*)& = J(K_N, b^{K_n}) -  J(K^*, b^*) + J(K_N, b_N) - J(K_N, b^{K_N})\\
& = J_1(K_N) - J_1(K^*) + J_2(K_N, b_N) - J_2(K_N, b^{K_N}). 
\$
Combining Theorem \ref{thm:ac_b} and the parameters chosen in the statement of this theorem, to show that $J(K_N, b_N) -  J(K^*, b^*) < \varepsilon$, we only need to prove that $J_1(K_N) -  J_1(K_*) < \varepsilon/2$. 

We proceed our proof by first showing the fact that $J_1(K)$ is gradient dominant, and then by using this fact to show the convergence of Algorithm \ref{algo:ac_lqr} combining the convergence result of policy evaluation in Theorem \ref{thm:pe}. 

To show that  $J_1(K)$ is gradient dominant, we first bound $J_1(K_1) - J_1(K_2)$ for any policy parameters $K_1$ and $K_2$.   Note that from Proposition \ref{prop:cost_form}, $J_1(K)$ takes the form
\$
J_1(K) = \tr(P_K \Psi_\epsilon) = \EE_{y\sim \mathcal N(0, \Psi_\epsilon)}(y^\top P_K y).
\$
To bound $J_1(K_1) - J_1(K_2)$ for any policy parameters $K_1$ and $K_2$, we use the following lemma to first bound $y^\top P_{K_1} y - y^\top P_{K_2} y$. 

\begin{lemma}\label{lemma:cost_diff}
Denote by $K_1$ and $K_2$ two policy parameters, which satisfy that $\rho(A-BK_1) < 1$ and $\rho(A-BK_2) < 1$. Moreover, for any state $y$, we denote by $\{y_t\}_{t\geq 0}$ the sequence generated by the dynamics $y_{t+1} = (A-BK_2)y_t$ with initial state $y_0 = y$. Then it satisfies that
\$
y^\top P_{K_2} y - y^\top P_{K_1} y = \sum_{t\geq 0} D_{K_1, K_2}(y_t).
\$
Here we denote by the function
\$
D_{K_1, K_2}(y) = 2y^\top (K_2 - K_1)(\Upsilon_{K_1}^{22} K_1  - \Upsilon_{K_1}^{21}) y + y^\top (K_2 - K_1)^\top\Upsilon_{K_1}^{22} (K_2 - K_1)x, 
\$
where we recall that the matrix $\Upsilon_K$ is defined in \eqref{eq:def_upsilon}. 
\end{lemma}
\begin{proof}
Please see \S\ref{proof:lemma:cost_diff}. 
\end{proof}

Now, based on the above Lemma \ref{lemma:cost_diff}, the following lemma shows that $J_1(K)$ is gradient dominant. 

\begin{lemma}\label{lemma:grad_dom}
Let $K^*$ be an optimal policy parameter and $K$ be a policy parameter such that $J_1(K)$ is finite, then we have the following lower bound for $J_1(K) - J_1(K^*)$:
\$
J_1(K) - J_1(K^*) \geq \sigma_{\min}(\Psi_\omega)\cdot \| \Upsilon_{K}^{22} \|_*^{-1}\cdot \tr\bigl[ (\Upsilon_K^{22} K  - \Upsilon_K^{21})^\top (\Upsilon_K^{22} K  - \Upsilon_K^{21}) \bigr],
\$ 
and the following upper bound:
\$
J_1(K) - J_1(K^*) \leq \sigma_{\min}^{-1}(R)\cdot \| \Phi^x_{K^*} \|_*\cdot \tr\bigl[ (\Upsilon_K^{22} K  - \Upsilon_K^{21})^\top (\Upsilon_K^{22} K  - \Upsilon_K^{21}) \bigr]. 
\$
\end{lemma}
\begin{proof}
Please see \S\ref{proof:lemma:grad_dom}. 
\end{proof}

By the upper established in Lemma \ref{lemma:grad_dom}, we can see that the difference $J_1(K) - J_1(K^*)$ is upper bounded by the natural gradient $\Upsilon_K^{22} K  - \Upsilon_K^{21}$.  

We now proceed to use the above results to show the convergence of Algorithm \ref{algo:ac_lqr}. Recall that according to Algorithm \ref{algo:ac_lqr}, the policy parameter $K$ is updated through the follows
\#\label{eq:ac_update_Kn}
K_{n + 1} = K_n - \gamma \cdot (\hat \Upsilon_{K_n}^{22}K_n - \hat \Upsilon_{K_n}^{21}),
\#
where $\hat \Upsilon_{K_n}$ is the output of Algorithm \ref{algo:pg_eval}.  We also define $\tilde K_{n+1}$ as an exact update: 
\#\label{eq:tilde_update_Kn}
\tilde K_{n+1} = K_n - \gamma \cdot ( \Upsilon_{K_n}^{22}K_n - \Upsilon_{K_n}^{21}),
\#
where $\Upsilon_{K_n}$ is given in \eqref{eq:def_upsilon}.    We proceed to bound $|J_1(K_{n+1}) - J_1(K^*)|$ in the sequel.  First, we use mathematical induction to show that the sequence $\{ J_1(K_n) \}_{n\geq 0}$ is non-increasing with large probability, as long as $J_1(K_n) - J_1(K^*)\geq \varepsilon/2$. Suppose that $J_1(K_n)\leq J_1(K_{n-1})\leq  \cdots \leq J_1(K_0)$ (note that this holds for $n=0$). 

Note that by the definition of $J_1(K)$ given in \eqref{eq:a2},  we have
\#\label{eq:diff_tildeK_K1}
& J_1(\tilde K_{n+1}) - J_1(K_n) = \EE_{y\sim\mathcal N(0, \Psi_\epsilon)}\bigl[ y^\top ( P_{\tilde K_{n+1}} - P_{K_n} )y \bigr]\notag\\
&\qquad = -2\gamma\cdot \tr\bigl[ \Phi^x_{\tilde K_{n+1}} \cdot (\Upsilon_{K_n}^{22}K_n - \Upsilon_{K_n}^{21})^\top (\Upsilon_{K_n}^{22}K_n - \Upsilon_{K_n}^{21}) \bigr] \notag\\
&\qquad\qquad+ (\gamma)^2\cdot \tr\bigl[ \Phi^x_{\tilde K_{n+1}} \cdot (\Upsilon_{K_n}^{22}K_n - \Upsilon_{K_n}^{21})^\top \Upsilon_{K_n}^{22}(\Upsilon_{K_n}^{22}K_n - \Upsilon_{K_n}^{21}) \bigr]\notag\\
&\qquad \leq -2\gamma\cdot \tr\bigl[ \Phi^x_{\tilde K_{n+1}} \cdot (\Upsilon_{K_n}^{22}K_n - \Upsilon_{K_n}^{21})^\top (\Upsilon_{K_n}^{22}K_n - \Upsilon_{K_n}^{21}) \bigr] \notag\\
& \qquad\qquad + (\gamma)^2\cdot \|\Upsilon_{K_n}^{22}\|_* \cdot \tr\bigl[ \Phi^x_{\tilde K_{n+1}} \cdot (\Upsilon_{K_n}^{22}K_n - \Upsilon_{K_n}^{21})^\top (\Upsilon_{K_n}^{22}K_n - \Upsilon_{K_n}^{21}) \bigr],
\#
where the second line comes from Lemma \ref{lemma:cost_diff}. Note that by the definition of $\Upsilon$ in \eqref{eq:def_upsilon}, we can upper bound $\|\Upsilon_{K_n}^{22}\|_*$ in the sequel:
\$
 \|\Upsilon_{K_n}^{22}\|_* & \leq \|R\|_* + \|B\|_*^2\cdot \|P_{K_n}\|_* \leq \|R\|_* + \|B\|_*^2\cdot J_1(K_n)\cdot \sigma_{\min}^{-1}(\Psi_\epsilon)\notag\\
& \leq \|R\|_* + \|B\|_*^2\cdot J_1(K_0)\cdot \sigma_{\min}^{-1}(\Psi_\epsilon). 
\$
Furthermore, combining \eqref{eq:diff_tildeK_K1} and the fact that the stepsize $\gamma\leq [\|R\|_* + \|B\|_*^2\cdot J_1(K_0)\cdot \sigma_{\min}^{-1}(\Psi_\epsilon)]^{-1}$,  it holds that
\#\label{eq:main_diff_J1}
J_1(\tilde K_{n+1}) - J_1(K_n)& \leq -\gamma\cdot \tr\bigl[ \Phi^x_{\tilde K_{n+1}} \cdot (\Upsilon_{K_n}^{22}K_n - \Upsilon_{K_n}^{21})^\top (\Upsilon_{K_n}^{22}K_n - \Upsilon_{K_n}^{21}) \bigr]\notag\\
&\leq -\gamma\cdot \sigma_{\min}(\Psi_\epsilon)\cdot  \tr\bigl[ (\Upsilon_{K_n}^{22}K_n - \Upsilon_{K_n}^{21})^\top (\Upsilon_{K_n}^{22}K_n - \Upsilon_{K_n}^{21}) \bigr]\notag\\
& \leq -\gamma\cdot \sigma_{\min}(\Psi_\epsilon)\cdot \sigma_{\min}(R)\cdot \|\Phi_{K^*}^x\|_*^{-1}\cdot  \bigl[ J_1(K_n) - J_1(K^*) \bigr],
\#
where the last line comes from Lemma \ref{lemma:grad_dom}. This also implies that $J_1(\tilde K_{n+1})\leq J_1(K_n)$. 

Now, we use the following lemma to establish the error bound $|J_1(\tilde K_{n+1}) - J_1( K_{n+1})|$. 

\begin{lemma}\label{lemma:error_bound_tilde_J}
Suppose that $J_1(K_n)\leq J_1(K_0)$.  Under the conditions stated in Theorem \ref{thm:ac}, with probability at least $1-\varepsilon^{10}$, it holds that
\$
\bigl|J_1(\tilde  K_{n+1}) - J_1( K_{n+1})\bigr| \leq \gamma\cdot \sigma_{\min}(\Psi_\epsilon)\cdot \sigma_{\min}(R)\cdot \|\Phi_{K^*}^x\|_*^{-1}\cdot  \varepsilon / 4, 
\$
where $K_{n+1}$ is generated from \eqref{eq:ac_update_Kn} and $\tilde K_{n+1}$ comes from \eqref{eq:tilde_update_Kn}. 
\end{lemma}
\begin{proof}
Please see \S\ref{proof:lemma:error_bound_tilde_J}. 
\end{proof}

Now, by applying the above Lemma \ref{lemma:error_bound_tilde_J}, we know that  if $J_1(K_n) - J_1(K^*) \geq \varepsilon/2$, combining \eqref{eq:main_diff_J1} and \eqref{eq:main_diff_J2}, it holds with probability at least $1-\varepsilon^{10}$ that
\#\label{eq:main_diff_J3}
J_1(K_{n+1}) - J_1(K_n) \leq - \gamma\cdot \sigma_{\min}(\Psi_\epsilon)\cdot \sigma_{\min}(R)\cdot \|\Phi_{K^*}^x\|_*^{-1}\cdot  \varepsilon / 4 < 0. 
\#
By this, we finish the mathematical induction that $\{ J_1(K_n) \}_{n\geq 0}$ is non-increasing with large probability, as long as $J_1(K_n) - J_1(K^*)\geq \varepsilon/2$.  

Also, when $J_1(K_n) - J_1(K^*)\geq \varepsilon/2$,  by \eqref{eq:main_diff_J1} and \eqref{eq:main_diff_J3}, with probability at least $1-\varepsilon^{10}$, it holds that
\$
J_1(K_{n+1}) - J_1(K^*) \leq \bigl[1-\gamma\cdot \sigma_{\min}(\Psi_\epsilon)\cdot \sigma_{\min}(R)\cdot \|\Phi_{K^*}^x\|_*^{-1}\bigr]\cdot  \bigl[ J_1(K_n) - J_1(K^*) \bigr],
\$ 
which proves the linear convergence rate of our proposed Algorithm \ref{algo:ac_lqr}. 

If suffices to give an error bound of $\|K_{n} - K^*\|_\F$.  We upper bound $\|K - K^*\|_\F$ using $J_1(K) - J_1(K^*)$ in the following lemma. 

\begin{lemma}\label{lemma:local_sc}
For any policy parameter $K$, we have
\$
\|K - K^*\|_\F^2 \leq \sigma_{\min}^{-1}(\Psi_\epsilon)\cdot \sigma_{\min}^{-1}(R) \cdot \bigl[ J_1(K) - J_1(K^*) \bigr]. 
\$
\end{lemma}
\begin{proof}
Please see \S\ref{proof:lemma:local_sc}. 
\end{proof}

Combining the above Lemma \ref{lemma:local_sc}, we conclude the theorem. 
\end{proof}

\subsection{Proof of Theorem \ref{thm:uniq_eq}}\label{proof:thm:uniq_eq}
\begin{proof}
We first compute the Lipschitz constants for both mappings $\cT_1(\cdot)$ and $\cT_2(\cdot, \cdot)$ in the sequel.

\textbf{Lipschitz constant for $\cT_1(\cdot)$. }   Note that by Proposition \ref{prop:J2}, for any $\mu_1, \mu_2\in\RR^d$, the induced optimal parameter policy $K^*$ is fixed for the problem \eqref{eq:slqr}. Therefore, it holds that
\#\label{eq:lip1}
\bigl\| \cT_1(\mu_1) - \cT_1(\mu_2)  \bigr\|_2 & \leq    \Bigl\| \bigl[ (I-A)Q^{-1}(I-A)^\top + BR^{-1}B^\top \bigr]^{-1} \overline A \Bigr\|_*\notag\\
& \qquad \cdot  \Bigl\| \bigl[ K^*Q^{-1} (I-A)^\top - R^{-1}B^\top \bigr]  \Bigr\|_* \cdot \|\mu_1 - \mu_2\|_2\notag\\
& =  L_1\cdot \|\mu_1 - \mu_2\|_2. 
\#

\textbf{Lipschitz constants for $\cT_2(\cdot, \cdot)$. }   Note that by Proposition \ref{prop:J2}, for any $\mu_1, \mu_2\in\RR^d$, the induced  optimal parameter policy $K^*$ is fixed for the problem \eqref{eq:slqr}. We thus have for any $\pi\in\Pi$, it holds that
\#\label{eq:lip2}
\bigl \| \cT_2(\mu_1, \pi) - \cT_2(\mu_2, \pi) \bigr\|_2& =  \bigl\|(I-A+BK_\pi)^{-1}\cdot \overline A\cdot (\mu_1-\mu_2) \bigr\|_2\notag\\
& \leq \bigl[1-\rho(A-BK^*)\bigr]^{-1}\|\overline A\|_*\cdot \|\mu_1 - \mu_2\|_2\notag\\
& =  L_2\cdot \|\mu_1 - \mu_2\|_2. 
\#
Moreover, for any $\pi_1, \pi_2\in\Pi$, and any population mean $\mu\in\RR^d$, we have
\#\label{eq:lip3}
\bigl \| \cT_2(\mu, \pi_1) - \cT_2(\mu, \pi_2) \bigr\|_2& =  \bigl\|(I-A+BK^*)^{-1} B\cdot (b_{\mu_1}-b_{\mu_2}) \bigr\|_2\notag\\
& \leq \bigl[1-\rho(A-BK^*)\bigr]^{-1}\|B\|_*\cdot \|b_{\mu_1}-b_{\mu_2}\|_2\notag\\
& = L_3\cdot \| \pi_1 - \pi_2 \|_2. 
\#

Now we show that the operator is a contraction.  For any $\mu_1, \mu_2\in\RR^d$, the following inequality holds:
\$
&\bigr\|\cT(\mu_1) - \cT(\mu_2)\bigr\|_2  = \Bigr\|\cT_2\bigl(\mu_1, \cT_1(\mu_1)\bigr) - \cT_2\bigl(\mu_2, \cT_1(\mu_2)\bigr)\Bigr\|_2\\
&\qquad \leq \Bigr\|\cT_2\bigl(\mu_1, \cT_1(\mu_1)\bigr) - \cT_2\bigl(\mu_1, \cT_1(\mu_2)\bigr)\Bigr\|_2 + \Bigr\|\cT_2\bigl(\mu_1, \cT_1(\mu_2)\bigr) - \cT_2\bigl(\mu_2, \cT_1(\mu_2)\bigr)\Bigr\|_2\\
& \qquad \leq L_3\cdot  \bigr\|\cT_1(\mu_1) -  \cT_1(\mu_2) \bigr\|_2 + L_2 \cdot \|\mu_1 - \mu_2\|_2 \\
& \qquad \leq L_3\cdot L_1\cdot \|\mu_1 - \mu_2\|_2 + L_2 \cdot \|\mu_1 - \mu_2\|_2 = (L_1L_3 + L_2)\cdot \|\mu_1 - \mu_2\|_2,
\$
where in the second line, we use triangular inequality; in the third line, we use \eqref{eq:lip2} and \eqref{eq:lip3}; in the last line, we use \eqref{eq:lip1}. By Assumption \ref{assum:contraction}, we know that $L_0 = L_1L_3 + L_2 < 1$, which shows that the operator $\cT(\cdot)$ is a contraction.  Therefore, by Banach fixed-point theorem, we conclude that $\cT(\cdot)$ has a unique fixed point, which gives the equilibrium pair of the problem \eqref{eq:mflqr}. 
\end{proof}

\subsection{Proof of Theorem \ref{thm:conv_mfg}}\label{proof:thm:conv_mfg}
\begin{proof}
We denote by $\mu_{s+1}^* = \cT(\mu_s)$, which gives the exact next population mean generated by the optimal policy $\cT_1(\mu_s)$ under the current population mean $\mu_s$. Then by \eqref{eq:f2q}, we know that
\$
\mu^*_{s + 1} = (I-A+BK^*)^{-1}\cdot \bigl[B b^*(\mu_s) + \overline A \mu_s\bigr],
\$
where $K^*$ and $b^*(\mu_s)$ are the optimal policy parameters under population mean $\mu_s$.  Further, we denote by
\$
\tilde \mu_{s+1} = (I-A + BK_s)^{-1} (Bb_s + \overline A\mu_s),
\$
which represents the population mean generated by the policy $\pi_s = (K_s, b_s)$.  According to our Algorithm \ref{algo:mflqr}, we can see that the output $\mu_{s+1}$ is actually a sample mean of $\tilde \mu_{s+1}$. 
Then we have
\#\label{eq:3terms}
\|\mu_{s+1} - \mu^*\|_2& \leq \| \mu_{s + 1} - \tilde \mu_{s+1}\|_2 + \| \tilde \mu_{s + 1} -  \mu^*_{s+1}\|_2 + \| \mu_{s+1}^* - \mu^*  \|_2   =: E_1 + E_2 + E_3. 
\#
We now proceed to bound the three terms $E_1$, $E_2$ and $E_3$ in the sequel. 

\textbf{Bound on $E_1$: }  Note that from the choice of the parameters in Algorithm \ref{algo:pg_eval} and Lemma \ref{lemma:dist_hat_muz}, it holds that
\#\label{eq:term1bound}
E_1 = \|\mu_{s+1} - \tilde \mu_{s+1}\|_2  < \varepsilon_s  \leq \varepsilon / 8 \cdot 2^{-s},
\#
with probability at least $1 - \varepsilon^{10}$.  By this, we establish a bound of $\|\mu_{s+1} - \tilde \mu_{s+1}\|_2$. 

\textbf{Bound on $E_2$: }  Note that by definition, combining with triangular inequality, we have
\#\label{eq:term2bound1}
E_2 & =  \Bigl\|  (I-A + BK_s)^{-1} (Bb_s + \overline A\mu_s) -  (I-A+BK^*)^{-1}\cdot \bigl[B b^*(\mu_s) + \overline A \mu_s\bigr]  \Bigr\|_2\notag\\
& \leq \bigl\|B b^*(\mu_s)  + \overline A\mu_s  \bigr\|_2\cdot \Bigl\|  \bigl[ I-A+BK^* + B(K_s - K^*) \bigr]^{-1} - (I-A+BK^*)^{-1} \Bigr\|_*\notag\\
&\qquad + \bigl\|  (I-A+BK_s)^{-1}  \bigr\|_*\cdot \|B\|_* \cdot \bigl\|b_s - b^*(\mu_s)\bigr\|_2\notag\\
& \leq 2 \bigl\|B b^*(\mu_s)  + \overline A\mu_s  \bigr\|_2\cdot \bigl\|  (I-A+BK^*)^{-1} B (K_s - K^*) (I-A+BK^*)^{-1} \bigr\|_*\notag\\
&\qquad + \bigl\|  (I-A+BK_s)^{-1}  \bigr\|_*\cdot \|B\|_* \cdot \bigl\|b_s - b^*(\mu_s)\bigr\|_2\notag\\
& \leq 2 \bigl\|B b^*(\mu_s)  + \overline A\mu_s  \bigr\|_2\cdot \bigl[ 1 - \rho(A-BK_*) \bigr]^{-2}\cdot \|B\|_* \cdot \|K_s - K^*\|_*\notag\\
&\qquad + \bigl[ 1 - \rho(A-BK_0) \bigr]^{-1} \cdot \|B\|_* \cdot \bigl\|b_s - b^*(\mu_s)\bigr\|_2. 
\#
For the term $\|B b^*(\mu_s)  + \overline A\mu_s \|_2$, combining Proposition \ref{prop:J2}, we know that 
\#\label{eq:term2bound2}
\bigl\|B b^*(\mu_s)  + \overline A\mu_s  \bigr\|_2 \leq L_1\cdot\|B\|_*\cdot \|\mu_s\|_2 + \|\overline A\|_*\cdot \|\mu_s\|_2 \leq  \bigl( \|B\|_* + \|\overline A\|_*\bigr) \cdot \|\mu_s\|_2,
\#
where the scalar $L_1$ is given in Assumption \ref{assum:contraction}.  Moreover, from Theorem \ref{thm:ac}, it holds with probability at least $1-\varepsilon^{10}$ that
\#\label{eq:term2bound3}
\|K_s - K^*\|_\F\leq \sqrt{\sigma_{\min}^{-1}(\Psi_\epsilon)\cdot \sigma_{\min}^{-1}(R) \cdot \varepsilon_s}, \qquad \bigl\|b_s - b^*(\mu_s)\bigr\|_2\leq \sqrt{2\nu_{K^*}^{-1}\cdot \varepsilon_s }. 
\#
Combining \eqref{eq:term2bound1}, \eqref{eq:term2bound2}, \eqref{eq:term2bound3} and the choice of $\epsilon_s$ in \eqref{eq:def_eps_s}, we deduce that 
\#\label{eq:term2bound}
E_2 \leq \varepsilon/8 \cdot 2^{-s}
\#
holds with probability at least $1-\varepsilon^{10}$. 

\textbf{Bound on $E_3$: }  We have
\#\label{eq:term3bound}
E_3 = \| \mu_{s+1}^* - \mu^*  \|_2 = \bigl\| \cT(\mu_{s}) - \cT(\mu^*)  \bigr\|_2\leq L_0\cdot  \| \mu_{s} - \mu^*  \|_2,
\#
where we use the fact that the operator $\cT(\cdot)$ has Lipschitz constant $L_0 = L_1L_3 + L_2$ according to Theorem \ref{thm:uniq_eq}. 

From \eqref{eq:term1bound}, \eqref{eq:term2bound} and \eqref{eq:term3bound}, combining \eqref{eq:3terms}, we know that 
\#\label{eq:iter1}
\|\mu_{s+1}-\mu^*\|_2 \leq   L_0\cdot \|\mu_{s}-\mu^*\|_2 + \varepsilon\cdot 2^{-s-2}.
\#
By telescoping \eqref{eq:iter1}, we obtain that
\$
\|\mu_S - \mu^*\|_2 \leq L_0^S\cdot \|\mu_0 - \mu^*\|_2 + \varepsilon/2. 
\$
Moreover, by the choice of $S$ in \eqref{eq:choice_S}, we know that $\|\mu_S - \mu^*\| < \varepsilon$. This concludes the theorem. 
\end{proof}

\section{Proofs of Propositions}
\subsection{Proof of Proposition \ref{prop:cost_form}}\label{proof:prop:cost_form}
\begin{proof}
By the definition of the cost $c_t$ defined in \eqref{eq:slqr}, we have
\#\label{eq:f4}
\EE c_t& = \EE(x_t^\top Q x_t  + u_t^\top R u_t + \mu^\top \overline Q \mu)\notag\\
& = \EE(x_t^\top Q x_t  + x_t^\top K^\top R K x_t - 2b^\top RK x_t + b^\top R b + \sigma^2 \eta_t^\top R\eta_t + \mu^\top \overline Q \mu)\notag\\
& = \EE\bigl[ x_t^\top(Q + K^\top R K) x_t - 2b^\top RK x_t \bigr] + b^\top R b + \sigma^2\cdot \tr(R) + \mu^\top \overline Q \mu,
\#
where in the second line we use the form of the linear policy defined in \eqref{eq:linear_policy}. Therefore, combining \eqref{eq:f4} and the definition of $J(K,b)$ in \eqref{eq:slqr}, we have
\$
J(K,b)& = \lim_{T\to\infty} \frac{1}{T}\sum_{t = 0}^T \Bigl\{ \EE\bigl[ x_t^\top(Q + K^\top R K) x_t  - 2b^\top RK x_t\bigr] + b^\top R b + \mu^\top \overline Q \mu \Bigr\}\notag\\
& = \EE_{x\sim\mathcal N(\mu_{K,b}^x, \Phi_K^x)}\bigl[ x^\top(Q + K^\top R K) x  - 2b^\top R K x \bigr] + b^\top R b + \sigma^2\cdot \tr(R) + \mu^\top \overline Q \mu\notag\\
& = \tr\bigl[(Q + K^\top R K)\Phi_K^x\bigr] + (\mu_{K,b}^x)^\top (Q+K^\top RK)\mu_{K,b}^x - 2b^\top RK\mu_{K,b}^x + b^\top Rb + \sigma^2\cdot \tr(R) + \mu^\top \overline Q\mu.
\$
Now, by applying \eqref{eq:f2p} and \eqref{eq:bellman} recursively, we have
\#\label{eq:f5}
\tr\bigl[(Q + K^\top R K)\Phi_K^x\bigr] = \tr(P_K\Psi_\epsilon),
\#
where $P_K$ is defined in \eqref{eq:bellman}. This finishes the proof of the proposition. 
\end{proof}

\subsection{Proof of Proposition \ref{prop:J2}}\label{proof:prop:J2}
\begin{proof}
Note that by the definition of $J_2(K,b)$ in \eqref{eq:a2} and the definition of $\mu_{K,b}^x$ in \eqref{eq:f2q}, the problem $\min_b J_2(K,b)$ is actually a constrained optimization program
\#\label{eq:a4}
\min_{\mu_{K,b}^x, b}&~ \begin{pmatrix}
\mu_{K,b}^x\\
b
\end{pmatrix}^\top
\begin{pmatrix}
Q+K^\top RK & -K^\top R\\
-RK & R
\end{pmatrix}
\begin{pmatrix}
\mu_{K,b}^x\\
b
\end{pmatrix}\notag\\
\text{s.t.} &~ (I-A+BK)\mu_{K,b}^x - (Bb+\overline{A}\mu) = 0. 
\#
Consider the KKT condition of the program \eqref{eq:a4}, the minimizer satisfies that
\#\label{eq:a5}
 2M_K
\begin{pmatrix}
\mu_{K,b^K}^x\\
b^K
\end{pmatrix}
+
N_K \lambda = 0, \qquad
 N_K^\top 
\begin{pmatrix}
\mu_{K,b^K}^x\\
b^K
\end{pmatrix} + \overline A \mu = 0,
\#
where we recall that
\$
M_K = \begin{pmatrix}
Q+K^\top RK & -K^\top R\\
-RK & R
\end{pmatrix}, \qquad N_K = \begin{pmatrix}
-(I-A+BK)^\top\\
B^\top
\end{pmatrix}. 
\$
By solving \eqref{eq:a5}, we obtain the minimizer to the program as follows
\#\label{eq:a7}
\begin{pmatrix}
\mu_{K,b^K}^x\\
b^K
\end{pmatrix}
 = -M_K^{-1}N_K (N_K^\top M_K^{-1}N_K)^{-1}\overline A\mu. 
\#
By substituting \eqref{eq:a7} into the expression of $J_2(K,b)$, we have
\#\label{eq:a8}
J_2(K,b^K) = \mu^\top \overline A^\top (N_K^\top M_K^{-1} N_K )^{-1}\overline A \mu. 
\#
Moreover, by algebra, we have
\$
M_K^{-1} = \begin{pmatrix}
Q^{-1} & Q^{-1}K^\top\\
K Q^{-1} & KQ^{-1}K^\top +R^{-1}
\end{pmatrix}. 
\$
Therefore, the term $N_K^\top M_K^{-1}N_K$ in \eqref{eq:a8} can be calculated as follows
\$
N_K^\top M_K^{-1}N_K = (I-A)Q^{-1}(I-A^\top) + BR^{-1}B^\top. 
\$
By substituting the above expression for $N_K^\top M_K^{-1}N_K$ into \eqref{eq:a8}, we have
\$
J_2(K, b^K) = \mu^\top \overline A^\top \bigl[ (I-A)Q^{-1}(I-A^\top) + BR^{-1}B^\top \bigr]^{-1} \overline A\mu.
\$
Also,  combining \eqref{eq:a7}, we also have
\$
\begin{pmatrix}
\mu_{K,b^K}^x\\
b^K
\end{pmatrix}
 = \begin{pmatrix}
 Q^{-1} (I-A)^\top\\
 KQ^{-1}(I-A)^\top - R^{-1}B^\top
 \end{pmatrix} \bigl[ (I-A)Q^{-1}(I-A)^\top + BR^{-1}B^\top \bigr]^{-1}  \overline A\mu. 
\$
Then we finish the proof of the proposition. 
\end{proof}

\subsection{Proof of Proposition \ref{prop:val_func_form}}\label{proof:prop:val_func_form}
\begin{proof}
From the definition of $V_{K,b}(x)$ in \eqref{eq:val_funcv}, we obtain that 
\$
V_{K,b}(x) = \sum_{t = 0}^\infty \Bigl\{ \EE\bigl[ & x_t^\top (Q+K^\top RK)x_t - 2b^\top RKx_t \\
& + b^\top Rb + \sigma^2 \eta_t^\top R\eta_t + \mu^\top \overline Q \mu \given x_0 = x\bigr] -J(K,b) \Bigr\}.
\$
Combining the linear dynamics in \eqref{eq:f1}, we can see that $V_{K,b}(x)$ is indeed a quadratic function taking the form $V_{K,b}(x) = x^\top G x + d^\top x + h$, where $G$, $d$ and $h$ are functions of $K$ and $b$. Moreover, note that $V_{K,b}(x)$ satisfies the Bellman equation, i.e., 
\$
V_{K,b}(x) = c(x,-Kx+b) - J(K,b) + \EE\bigl[ V_{K,b}(x')\given x \bigr].
\$
By substituting the form of $c(x,-Kx+b)$ given in \eqref{eq:slqr} and $J(K,b)$ given in \eqref{eq:a1}, we obtain that
\#\label{eq:f6}
x^\top G x + d^\top x + h =& x^\top (Q + K^\top RK)x - 2b^\top RKx + b^\top Rb + \mu^\top \overline Q \mu\notag\\
& - \bigl[ \tr(P_K \Psi_\epsilon) + (\mu_{K,b}^x)^\top (Q+K^\top RK)\mu_{K,b}^x - 2b^\top RK\mu_{K,b}^x + \mu^\top \overline Q \mu + b^\top Rb \bigr ]\notag\\
& + \bigl[ (A-BK)x + (Bb+\overline A\mu)  \bigr]^\top G \bigl[(A-BK)x + (Bb+\overline A\mu)  \bigr]\notag\\
& + \tr(G\Psi_\epsilon) + d^\top \bigl[ (A-BK)x + (Bb+\overline A\mu) \bigr] + h. 
\#
By comparing the quadratic term and linear term in \eqref{eq:f6}, we obtain that
\$
G = P_K, \qquad d = 2f_{K,b}.
\$
Moreover, by the definition of $V_{K,b}(x)$ in \eqref{eq:val_funcv}, we know that $\EE[V_{K,b}(x)] = 0$, therefore, we have
\$
h = -2f_{K,b}\mu_{K,b}^x - (\mu_{K,b}^x)^\top P_K\mu_{K,b}^x - \tr(P_K\Phi_K^x). 
\$
This finishes the proof of \eqref{eq:4a}. 

As for the state-action value function $Q_{K,b}(x,u)$, by applying the definition in \eqref{eq:val_funcq} straightforwardly, we obtain \eqref{eq:4b}. This finishes the proof of the proposition. 
\end{proof}

\subsection{Proof of Proposition \ref{prop:bellman_compact}}\label{proof:prop:bellman_compact}
\begin{proof}
Given the ergodic cost, recall that the Bellman equation takes the form
\#\label{eq:q4}
Q_{K,b}(x,u) = c(x,u) - J(K,b) + \EE_{\pi_{K,b}}\bigl[ Q_{K,b}(x',u')\given x,u \bigr],
\#
where $(x',u')$ is the state-action pair after $(x,u)$. Also, note that the state-action value function also takes the form stated in \eqref{eq:q3}, by plugging \eqref{eq:q3} into \eqref{eq:q4}, we obtain that
\#\label{eq:q5}
 \psi(x,u)^\top \alpha_{K,b}  =  c(x,u) - J(K,b) +  \EE_{\pi_{K,b}}\bigl[\psi(x',u')\given x,u\bigr]^\top \alpha_{K,b}.
\#
By left multiplying $\psi(x,u)$ to both sides of \eqref{eq:q5}, and taking the total expectation, we have
\$
\EE_{\pi_{K,b}}\Bigl\{ \psi(x,u) \bigl[\psi(x,u) -\psi(x',u')\bigr]^\top \Bigr \} \cdot \alpha_{K,b} + \EE_{\pi_{K,b}}\bigl[ \psi(x,u)\bigr] \cdot J(K,b)  =  \EE_{\pi_{K,b}}\bigl[c(x,u) \psi(x,u)\bigr]. 
\$
Combining the definition of the matrix $\Theta_{K,b}$ in \eqref{eq:q2}, we conclude the proposition. 
\end{proof}

\subsection{Proof of Proposition \ref{prop:invert_theta}}\label{proof:prop:invert_theta}
\begin{proof}

\textbf{Invertibility: }
we define the concatenate $z = (x^\top, u^\top)^\top$, then the transition of $z$ takes the form
\$
z' = Lz + \nu + \delta,
\$
where the matrix $L$ and the vectors $\nu$, $\delta$ are defined as
\$
\nu = \begin{pmatrix}
\overline A \mu\\
-K\overline A\mu + b
\end{pmatrix}, \qquad
\delta = \begin{pmatrix}
\omega\\
-K\omega + \sigma \eta
\end{pmatrix},\qquad
L = \begin{pmatrix}
A & B\\
-KA & -KB
\end{pmatrix}. 
\$
Note that by observation we can write
\$
L = \begin{pmatrix}
I\\
-K
\end{pmatrix}
\begin{pmatrix}
A & B
\end{pmatrix}. 
\$
Combining the fact that $\rho(UV) = \rho(VU)$ for any matrices $U$ and $V$, we obtain that $\rho(L) = \rho(A-BK) < 1$. 

Note that by the transition, we can see that the mean $\mu_z$ and the covariance $\Sigma_z$ satisfy the following Lyapunov equations
\#\label{eq:lyap}
\mu_z = L\mu_z + \nu, \qquad \Sigma_z = L\Sigma_z L^\top  + \Psi_\delta,
\#
where the matrix $\Psi_\delta$ is the covariance of the vector $\delta$, which takes the form
\$
\Psi_\delta = \begin{pmatrix}
\Psi_\omega & -\Psi_\omega K^\top\\
-K \Psi_\omega & K\Psi_\omega K^\top +\sigma^2 I 
\end{pmatrix}. 
\$
Moreover, the covariance matrix $\Sigma_z$ can be written explicitly in the following way:
\#\label{eq:sigma_z_factor}
\Sigma_z = \begin{pmatrix}
\Phi_K^x & -\Phi_K^x K^\top\\
-K\Phi_K^x & K\Phi_K^x K^\top + \sigma^2 \cdot I
\end{pmatrix} = \begin{pmatrix}
0 & 0\\
0 & \sigma^2\cdot I
\end{pmatrix} + \begin{pmatrix}
I\\
-K
\end{pmatrix}\Phi_K^x\begin{pmatrix}
I\\
-K
\end{pmatrix}^\top. 
\#

Now, based on the above notations, we establish the following lemma to calculate $\Theta_{K,b}$. 

\begin{lemma}\label{lemma:theta_form}
Under the notations above, the matrix $\Theta_{K,b}$ defined in \eqref{eq:q2} takes the following form
\#\label{eq:form_Theta}
\Theta_{K,b} = \begin{pmatrix}
2 (\Sigma_z\otimes_s \Sigma_z) (I - L \otimes_s L)^\top & 0 \\
0 & \Sigma_z (I-L)^\top
\end{pmatrix}. 
\#
\end{lemma}
\begin{proof}
Please see \S\ref{proof:lemma:theta_form}. 
\end{proof}

Note that since $\rho(L) < 1$, both the matrices $I-L \otimes_s L$ and $I-L$ are positive definite; therefore, by the above Lemma \ref{lemma:theta_form}, the matrix $\Theta_{K,b}$ is invertible. This finishes the proof of the invertibility of the matrix $\Theta_{K,b}$.  Moreover, from \eqref{eq:sigma_z_factor} and Lemma \ref{lemma:theta_form}, we can upper bound the spectral norm of $\Theta_{K,b}$ as follows
\$
\|\Theta_{K,b}\|_* & \leq 2 \max\Bigl\{ \|\Sigma_z\|_*^2\cdot \bigl(1 + \|L\|_*^2\bigr),~ \|\Sigma_z\|_*\cdot \bigl(1 + \|L\|_*\bigr) \Bigr \} \\
& \leq 4\|\Sigma_z\|_*^2\leq 4 \bigl( 1 + \|K\|_\F^2 \bigr)^2\cdot \|\Phi_K^x\|_*^2. 
\$
This proves the first part of the proposition. 

\textbf{Minimum singular value: } recall that the matrix $\tilde \Theta_{K,b}$ in the linear system \eqref{eq:linear_sys} takes the following form 
\$
\tilde \Theta_{K,b} = \begin{pmatrix}
1 & 0\\
\EE_{\pi_{K,b}}\bigl[ \psi(x,u)  \bigr] & \Theta_{K,b}
\end{pmatrix}. 
\$
By the definition of the feature vector $\psi(x,u)$, it is straightforward to verify that the vector $\tilde \sigma_z = \EE_{\pi_{K,b}}[ \psi(x,u) ]$ takes the form
\#\label{eq:tilde_sigma}
\tilde \sigma_z = \EE_{\pi_{K,b}}\bigl[ \psi(x,u) \bigr] = \begin{pmatrix}
\svec(\Sigma_z)\\
\mathbf 0_{k+d}
\end{pmatrix}, 
\#
where $\mathbf 0_{k+d}$ denotes the all-zero column vector with dimension $k+d$. Also, note that since the matrix $\Theta_{K,b}$ is invertible, the block matrix $\tilde \Theta_{K,b}$ is also invertible, and simple calculation gives its inverse as follows
\$
\tilde \Theta_{K,b}^{-1} = \begin{pmatrix}
1 & 0\\
-\Theta_{K,b}^{-1}\cdot  \tilde \sigma_z & \Theta_{K,b}^{-1}
\end{pmatrix}. 
\$

The following lemma characterize the spectral norm of the matrix $\tilde \Theta_{K,b}^{-1}$. 

\begin{lemma}\label{lemma:upper_bound_tilde_theta}
The spectral norm of the matrix $\tilde \Theta_{K,b}^{-1}$ is upper bounded by some positive constant $\tilde \lambda_K$, where $\tilde \lambda_K$ only depends on $\rho(A-BK)$, $\sigma$ and $\sigma_{\min}(\Psi_\omega)$. 
\end{lemma}
\begin{proof}
Please see \S\ref{proof:lemma:upper_bound_tilde_theta}. 
\end{proof}

By the above Lemma \ref{lemma:upper_bound_tilde_theta}, we know that minimum singular value of the matrix $\tilde\Theta_{K,b}$ can be lower bounded by a positive constant $\lambda_K = 1/\tilde \lambda_K$, which only depends on $\rho(A-BK)$, $\sigma$ and $\sigma_{\min}(\Psi_\omega)$. This concludes the proposition. 
\end{proof}

\section{Proofs of Lemmas}
\subsection{Proof of Lemma \ref{lemma:theta_form}}\label{proof:lemma:theta_form}
\begin{proof}
Then by the above notations, the feature vector $\psi(x,u)$ takes the following form
\$
\psi(x,u) = \begin{pmatrix}
\svec\bigl[ (z-\mu_z)(z-\mu_z)^\top \bigr]\\
z-\mu_z
\end{pmatrix}.
\$
We then have
\$
\psi(x,u) - \psi(x',u') = \begin{pmatrix}
\svec\bigl[ yy^\top - (Ly +\delta)(Ly+\delta)^\top \bigr]\\
y - (Ly+\delta)
\end{pmatrix},
\$
where we denote by $y = z-\mu_z$.    Therefore, for any symmetric matrices $M$, $N$ and any vectors $m$, $n$,  the following equation holds
\#\label{eq:quad_deri}
& \begin{pmatrix}
\svec(M)\\
m
\end{pmatrix}^\top 
\Theta_{K,b}
\begin{pmatrix}
\svec(N)\\
n
\end{pmatrix}\notag \\
& \qquad = \EE_{y, \delta}\Biggl\{  \begin{pmatrix}
\svec(M)\\
m
\end{pmatrix}^\top   
\begin{pmatrix}
\svec(yy^\top)\\
y
\end{pmatrix}
\begin{pmatrix}
\svec\bigl[ yy^\top - (Ly +\delta)(Ly +\delta)^\top \bigr]\\
y - (Ly+\delta)
\end{pmatrix}^\top
\begin{pmatrix}
\svec(N)\\
n
\end{pmatrix} \Biggr \} \notag \\
&\qquad = \EE_{y, \delta}\Bigl\{ \bigl( \la M, yy^\top\ra + m^\top y\bigr)\cdot \bigl[  \la N,  yy^\top - (Ly+\delta)(Ly+\delta)^\top\ra  + n^\top (y-Ly-\delta)     \bigr]  \Bigr\}\notag \\
&\qquad = \underbrace{ \EE_{y}\bigl[  \la yy^\top, M\ra\cdot \la yy^\top -Lyy^\top L^\top - \Psi_\delta, N  \ra  \bigr] }_{A_1}  + \underbrace{ \EE_{y}\bigl[ \la yy^\top, M\ra\cdot n^\top (y-Ly)  \bigr] }_{A_2}\notag\\
&\qquad\qquad +  \underbrace{  \EE_{y}  \bigl[   m^\top y\cdot \la yy^\top -Lyy^\top L^\top - \Psi_\delta, N\ra   \bigr]   }_{A_3} + \underbrace{  \EE_{y}  \bigl[  m^\top y\cdot n^\top (y-Ly)  \bigr] }_{A_4},
\#
where the expectations are taken under the distribution $y\sim\mathcal N(0,\Sigma_z)$ and $\delta\sim\mathcal N(0,\Psi_\delta)$. 

For the terms $A_2$ and $A_3$ in \eqref{eq:quad_deri}, note that $y = z-\mu_z\sim\mathcal N (0,\Sigma_z)$, thus these two terms vanish.   For $A_4$, we calculate in the sequel:
\#\label{eq:cal_a4}
A_4 = \EE_y\bigl[ m^\top y\cdot (y-Ly)^\top n \bigr] = \EE_y\bigl[ m^\top y y^\top (I-L)^\top n \bigr] = m^\top \Sigma_z (I-L)^\top n. 
\#
For $A_1$, by algebra, we have
\#\label{eq:cal_a1_1}
A_1&  =   \EE_{y}\bigl[  \la yy^\top, M\ra\cdot \la yy^\top -Lyy^\top L^\top - \Psi_\delta, N  \ra  \bigr]\notag\\
& = \EE_{y}\bigl[  \la yy^\top, M\ra\cdot \la yy^\top -Lyy^\top L^\top, N  \ra  \bigr] - \EE_{y}\bigl[  \la yy^\top, M\ra\cdot  \la \Psi_\delta, N  \ra  \bigr]\notag\\
& = \EE_{y}\bigl[  y^\top M y \cdot y^\top (N-L^\top N L) y  \bigr] -  \la \Sigma_z, M\ra\cdot  \la \Psi_\delta, N  \ra \notag\\
& = \EE_{u\sim\mathcal N(0,I)}\bigl[  u^\top \Sigma_z^{1/2} M \Sigma_z^{1/2} u \cdot u^\top \Sigma_z^{1/2} (N-L^\top N L) \Sigma_z^{1/2} u  \bigr] -  \la \Sigma_z, M\ra\cdot  \la \Psi_\delta, N  \ra. 
\#
Here $\Sigma_z^{1/2}$ represents the square root of $\Sigma_z$, which is well-defined since the covariance matrix $\Sigma_z$ is positive definite.  
We now apply Lemma \ref{lemma:magnus} to the first term in \eqref{eq:cal_a1_1}, then we know that
\$
A_1 & = 2\tr\bigl[ \Sigma_z^{1/2} M \Sigma_z^{1/2}\cdot \Sigma_z^{1/2} (N-L^\top N L) \Sigma_z^{1/2} \bigr]\notag\\
&\qquad + \tr(\Sigma_z^{1/2} M \Sigma_z^{1/2})\cdot \tr\bigl[ \Sigma_z^{1/2} (N-L^\top N L) \Sigma_z^{1/2} \bigr] - \la \Sigma_z, M\ra\cdot  \la \Psi_\delta, N  \ra\notag\\
& = 2\la M, \Sigma_z (N-L^\top N L )\Sigma_z\ra + \la \Sigma_z, M\ra\cdot \la \Sigma_z - L\Sigma_z L^\top - \Psi_\delta, N\ra  \notag\\
&= 2\la M, \Sigma_z (N-L^\top N L )\Sigma_z\ra,
\$
where we use the Lyapunov equation \eqref{eq:lyap} in the last equality.   By using the property of the operator $\svec$ and the definition of the symmetric Kronecker product, we obtain that
\#\label{eq:cal_a1}
A_1& = 2\svec(M)^\top \svec\bigl[ \Sigma_z (N-L^\top N L )\Sigma_z \bigr]\notag\\
& = 2\svec(M)^\top \bigl[\Sigma_z\otimes_s \Sigma_z - (\Sigma_z L^\top) \otimes_s (\Sigma_z L^\top) \bigr]\svec(N)\notag\\
& = 2\svec(M)^\top \bigl[(\Sigma_z\otimes_s \Sigma_z)(I-L \otimes_s L)^\top \bigr]\svec(N). 
\#
Combining \eqref{eq:quad_deri}, \eqref{eq:cal_a1} and \eqref{eq:cal_a4}, we obtain that
\$
& \begin{pmatrix}
\svec(M)\\
m
\end{pmatrix}^\top 
\Theta_{K,b}
\begin{pmatrix}
\svec(N)\\
n
\end{pmatrix} \\
&\qquad =  \svec(M)^\top \bigl[2 (\Sigma_z\otimes_s \Sigma_z)(I-L \otimes_s L)^\top \bigr]\svec(N) +   m^\top \Sigma_z (I-L)^\top n. 
\$
Thus, we can write the matrix $\Theta_{K,b}$ in the following form
\$
\Theta_{K,b} = \begin{pmatrix}
2 (\Sigma_z\otimes_s \Sigma_z) (I - L \otimes_s L)^\top & 0 \\
0 & \Sigma_z (I-L)^\top
\end{pmatrix}. 
\$
This concludes the lemma. 
\end{proof}

\subsection{Proof of Lemma \ref{lemma:upper_bound_tilde_theta}}\label{proof:lemma:upper_bound_tilde_theta}
\begin{proof}
By the property of the spectral norm, we can bound the spectral norm of the above matrix $\tilde \Theta_{K,b}^{-1}$ as follows
\#\label{eq:norm_tilde}
\|\tilde \Theta_{K,b}^{-1} \|_*^2 \leq 1 + \|\Theta_{K,b}^{-1}\|_*^2 + \|\Theta_{K,b}^{-1}\tilde \sigma_z\|_2^2. 
\#
We proceed to bound each term on the RHS of \eqref{eq:norm_tilde}.   
For the term $\Theta_{K,b}^{-1}\tilde \sigma_z$, combining \eqref{eq:form_Theta} and \eqref{eq:tilde_sigma}, we have
\$
\Theta_{K,b}^{-1}\tilde \sigma_z & = \begin{pmatrix}
1/2\cdot  (I-L \otimes_s L) ^{-\top}  (\Sigma_z\otimes_s \Sigma_z)^{-1}\cdot \svec(\Sigma_z)\\
\mathbf 0_{k+d}
\end{pmatrix}\\
& = \begin{pmatrix}
1/2\cdot  (I-L \otimes_s L) ^{-\top}  (\Sigma_z^{-1}\otimes_s \Sigma_z^{-1} ) \cdot  \svec(\Sigma_z)\\
\mathbf 0_{k+d}
\end{pmatrix}\\
& = \begin{pmatrix}
1/2\cdot  (I-L \otimes_s L) ^{-\top} \cdot  \svec(\Sigma_z^{-1})\\
\mathbf 0_{k+d}
\end{pmatrix},
\$
where we use the property and the definition of the symmetric Kronecker product in the second and last line, respectively.  Therefore,  we  have
\#\label{eq:norm_theta_sigma}
\|\Theta_{K,b}^{-1}\tilde \sigma_z\|_2&  = 1/2\cdot \bigl \| (I-L \otimes_s L) ^{-\top} \cdot  \svec(\Sigma_z^{-1})\bigr \|_2\notag\\
& \leq 1/2\cdot \bigl \| (I-L \otimes_s L) ^{-\top} \bigr \|_* \cdot  \bigl \| \svec(\Sigma_z^{-1})\bigr \|_2\notag\\
& \leq 1/2\cdot \bigl[1-\rho^2(L)\bigr]^{-1}\cdot \|\Sigma_z^{-1}\|_\F\notag\\
& \leq 1/2\cdot\sqrt{k+d}\cdot \bigl[1-\rho^2(L)\bigr]^{-1}\cdot \|\Sigma_z^{-1}\|_*\notag\\
& = 1/2\cdot\sqrt{k+d}\cdot \bigl[1-\rho^2(L)\bigr]^{-1} \cdot  \bigl[\sigma_{\min} (\Sigma_z) \bigr]^{-1},
\# 
where in the third line we use Lemma \ref{lemma:alizadeh1998primal} to the matrix $L\otimes L$.  Similarly, we bound the spectral norm of $\Theta_{K,b}^{-1}$ in the sequel
\#\label{eq:norm_theta}
\|\Theta_{K,b}^{-1}\|_* \leq \min\Bigl\{  1/2\cdot \bigl[ 1-\rho^2(L) \bigr]^{-1} \bigl[\sigma_{\min} (\Sigma_z) \bigr]^{-2}, \bigl[ 1-\rho(L) \bigr]^{-1} \bigl[\sigma_{\min} (\Sigma_z) \bigr]^{-1} \Bigr\}. 
\#
Thus, combining \eqref{eq:norm_tilde}, \eqref{eq:norm_theta_sigma} and \eqref{eq:norm_theta}, we obtain that
\#\label{eq:norm_tilde2}
\|\tilde \Theta_{K,b}^{-1} \|_*^2  &\leq 1 + 1/2\cdot\sqrt{k+d}\cdot \bigl[1-\rho^2(L)\bigr]^{-1} \cdot  \bigl[\sigma_{\min} (\Sigma_z) \bigr]^{-1}\notag\\
&  \qquad +  \min\Bigl\{  1/2\cdot \bigl[ 1-\rho^2(L) \bigr]^{-1} \bigl[\sigma_{\min} (\Sigma_z) \bigr]^{-2}, \bigl[ 1-\rho(L) \bigr]^{-1} \bigl[\sigma_{\min} (\Sigma_z) \bigr]^{-1} \Bigr\}. 
\#
Now we proceed to characterize the lower bound of $\sigma_{\min}(\Sigma_z)$ in the sequel.  For any test vectors $s\in\RR^d$ and $r\in\RR^k$, by algebra, we have
\#\label{eq:quad_sigmaz}
\begin{pmatrix}
s\\
r
\end{pmatrix}^\top  \Sigma_z \begin{pmatrix}
s\\
r
\end{pmatrix} & = \EE_{\pi_{K,b}}\Bigl\{ \bigl[ s^\top (x-\mu_{K,b}^x) + r^\top (u+K\mu_{K,b}^x - b) \bigr]^2 \Bigr\} \notag\\
& = \EE_{x, \eta}\Bigl\{ \bigl[ (s-K^\top r)^\top (x-\mu_{K,b}^x) + \sigma r^\top \eta \bigr]^2 \Bigr\}\notag\\
& = \EE_{x}\Bigl\{ \bigl[ (s-K^\top r)^\top (x-\mu_{K,b}^x)  \bigr]^2 \Bigr\} + \EE_{\eta} \bigl[ ( \sigma r^\top \eta)^2 \bigr]. 
\#
For the first term on the RHS of \eqref{eq:quad_sigmaz}, we lower bound it as follows
\#\label{eq:quad_sigmaz1}
& \EE_{x}\Bigl\{ \bigl[ (s-K^\top r)^\top (x-\mu_{K,b}^x)  \bigr]^2 \Bigr\} = (s-K^\top r)^\top \Sigma_z (s-K^\top r)\notag\\
&\qquad \geq \|s-K^\top r\|_2^2\cdot \sigma_{\min}(\Phi_K^x) \geq \|s-K^\top r\|_2^2\cdot \sigma_{\min}(\Psi_\omega),
\#
where the last inequality comes from the fact that $\sigma_{\min}(\Phi_K^x)\geq \sigma_{\min}(\Psi_\omega)$ by \eqref{eq:f2p}.  Also, the second term on the RHS of \eqref{eq:quad_sigmaz} takes the form $\EE_{\eta} [ ( \sigma r^\top \eta)^2 ] = \sigma^2 \|r\|_2^2$. Therefore, combining \eqref{eq:quad_sigmaz} and \eqref{eq:quad_sigmaz1}, we have
\$
\begin{pmatrix}
s\\
r
\end{pmatrix}^\top  \Sigma_z \begin{pmatrix}
s\\
r
\end{pmatrix} & \geq \|s-K^\top r\|_2^2\cdot \sigma_{\min}(\Psi_\omega) + \sigma^2 \|r\|_2^2 \notag\\
&\geq \sigma_{\min}(\Psi_\omega)\cdot \|s\|_2^2 + \bigl[\sigma^2 -  \|K\|_*^2\cdot \sigma_{\min}(\Psi_\omega) \bigr]\cdot \|r\|_2^2. 
\$
From this, we can see that $\sigma_{\min}(\Sigma_z)$ is lower bounded by $\min\{ \sigma_{\min}(\Psi_\omega), \sigma^2 -  \|K\|_*^2\cdot \sigma_{\min}(\Psi_\omega)  \}$, which only depends on $\sigma_{\min}(\Psi_\omega)$ and $\sigma$. Thus, combining \eqref{eq:norm_tilde2}, it is straightforward to see that $\|\tilde \Theta_{K,b}^{-1}\|_*$ is upper bounded by some constant $\tilde \lambda_K$, where $\tilde \lambda_K$ only depends on $\rho(A-BK)$, $\sigma$ and $\sigma_{\min}(\Psi_\omega)$.   This finishes the proof of the lemma. 
\end{proof}

\subsection{Proof of Lemma \ref{lemma:zeta_xi}}\label{proof:lemma:zeta_xi}
\begin{proof}
\textbf{Part 1.} First we proceed to prove that $\zeta_{K,b}\in\cV_\zeta$. 
Note that from Assumption \ref{assum:proj}, we know that $\zeta_{K,b}^1 = J(K,b)$ satisfies that $0\leq \zeta_{K,b}^1 \leq J_0$.  It remains to show that $\zeta_{K,b}^2 = \alpha_{K,b}$ satisfies that $\|\zeta_{K,b}^2\|_2\leq M_\zeta$. By the definition of $\alpha_{K,b}$ in \eqref{eq:q1}, we know that
\#\label{eq:alpha_bound}
\|\alpha_{K,b}\|_2^2 &\leq \|\Upsilon_K\|_\F^2 + \|\Upsilon_K\|_*^2 \cdot \bigl( \|\mu_{K,b}^x\|_2^2 + \|\mu_{K,b}^u\|_2^2 \bigr) \notag\\
&\qquad + \bigl(\|A\|_* + \|B\|_*\bigr)^2\cdot \bigl(\|P_K\|_* \cdot \|\overline A \mu\|_2 + \|f_{K, b}\|_2\bigr)^2
\#
where for notational simplicity, we denote by $\mu_{K,b}^u$ the mean of action, i.e., $\mu_{K,b}^u = -K\mu_{K,b}^x + b$. We only need to bound $\Upsilon_K$, $\mu_{K,b}^x$, $\mu_{K,b}^u$, $P_K$ and $f_{K,b}$.  For $\mu_{K,b}^x$, $\mu_{K,b}^u$ and $P_K$, note that under the above notations, the total cost $J(K, b)$ actually takes the form
\$
J(K, b) = \tr(P_K\Psi_\epsilon) + (\mu_{K,b}^x)^\top Q\mu_{K,b}^x + (\mu_{K,b}^u)^\top R\mu_{K,b}^u + \sigma^2\cdot \tr(R) + \mu^\top \overline Q\mu. 
\$
Thus, we have
\$
& J_0\geq J(K, b)\geq \sigma_{\min}(\Psi_\omega)\cdot \tr(P_K) \geq \sigma_{\min}(\Psi_\omega)\cdot \|P_K\|_*, \\
& J_0\geq J(K, b)\geq (\mu_{K,b}^x)^\top Q\mu_{K,b}^x\geq \sigma_{\min}(Q)\cdot \|\mu_{K,b}^x\|_2, \\
& J_0\geq J(K, b)\geq (\mu_{K,b}^u)^\top R\mu_{K,b}^u\geq \sigma_{\min}(R)\cdot \|\mu_{K,b}^u\|_2, \\
\$
which imply that 
\#\label{eq:bound_mu_P}
\|P_K\|_*\leq J_0/\sigma_{\min}(\Psi_\omega), \qquad \|\mu_{K,b}^x\|_2\leq J_0/\sigma_{\min}(Q), \qquad \|\mu_{K,b}^u\|_2\leq J_0/\sigma_{\min}(R). 
\#
For $\Upsilon_K$, note that we can decompose the matrix in the following way:
\$
\Upsilon_K = \begin{pmatrix}
Q & \\
& R
\end{pmatrix}  +  \begin{pmatrix}
A^\top\\
B^\top
\end{pmatrix}P_K    \begin{pmatrix}
A & B
\end{pmatrix},
\$
which gives
\$
& \|\Upsilon_K\|_\F \leq (\|Q\|_\F + \|R\|_\F) + \bigl( \|A\|_\F^2 + \|B\|_\F^2 \bigr)\cdot \| P_K \|_\F, \notag\\
& \|\Upsilon_K\|_* \leq (\|Q\|_* + \|R\|_*) + \bigl( \|A\|_* + \|B\|_* \bigr)^2 \cdot \| P_K \|_*. 
\$
Combining \eqref{eq:bound_mu_P} and the fact that $\|U\|_\F\leq \sqrt{d}\cdot \|U\|_*$ for any $U\in\RR^{d\times d}$, we know that 
\#\label{eq:bound_upsilon}
& \|\Upsilon_K\|_\F \leq (\|Q\|_\F + \|R\|_\F) + \bigl( \|A\|_\F^2 + \|B\|_\F^2 \bigr)\cdot \sqrt{d}\cdot J_0/\sigma_{\min}(\Psi_\omega), \notag\\
& \|\Upsilon_K\|_* \leq (\|Q\|_* + \|R\|_*) + \bigl( \|A\|_* + \|B\|_* \bigr)^2 \cdot J_0/\sigma_{\min}(\Psi_\omega). 
\#
Now we focus on the bound of the vector $f_{K,b}$. 
\iffalse
Note that from the proof of Proposition \ref{prop:J2} in \S\ref{proof:prop:J2}, we derive an explicit form of $b^K$, which is given in \eqref{eq:a7}. Thus, by plugging \eqref{eq:a7} into the definition of $f_{K,b^K}$ proposed in Proposition \ref{prop:val_func_form}, we know that $f_{K, b^K}$ actually takes the following form
\$
f_{K,b^K} = \bigl[ I - P_K Q^{-1} (I-A)^\top \bigr] \cdot \bigl[ (I-A)Q^{-1} (I-A)^\top  + BR^{-1} B^\top \bigr]^{-1}\overline A\mu, 
\$
which gives the following bound on $f_{K, b^K}$ combining \eqref{eq:bound_mu_P}
\#\label{eq:bound_fKb}
\|f_{K,b^K}\|_2& \leq \bigl(1 +  J_0 /\sigma_{\min}(\Psi_\omega)\cdot \|Q^{-1}\|_* \|I-A\|_*\bigr)\notag\\
& \qquad \cdot \Bigl\|  \bigl[(I-A)Q^{-1}(I-A)^\top  + B R^{-1} B^\top \bigr]^{-1} \overline A\mu \Bigr\|_2. 
\#
\fi
Note that we can write $f_{K,b}$ in the following way
\$
f_{K,b} = -P_K\mu_{K,b}^x + (I-A+BK)^{-T}\bigl[ Q\mu_{K,b}^x - K^\top R\mu_{K,b}^u \bigr],
\$ 
we can therefore upper bound $f_{K,b}$ as
\#\label{eq:bound_fKb}
\|f_{K,b}\|_2\leq  J_0^2\cdot \sigma_{\min}^{-1}(\Psi_\omega)\cdot \sigma_{\min}^{-1}(Q) + \bigl[ 1-\rho(A-BK) \bigr]^{-1}\cdot(\kappa_Q + \kappa_R\cdot \|K\|_\F)
\#
Combining \eqref{eq:alpha_bound}, \eqref{eq:bound_mu_P}, \eqref{eq:bound_upsilon} and \eqref{eq:bound_fKb}, we know that $\|\zeta_{K,b^K}^2\|_2 = \|\alpha_{K,b^K}\|_2 \leq M_{\zeta,1} + M_{\zeta,2}\cdot(1+ \|K\|_\F)\cdot [ 1-\rho(A-BK) ]^{-1}$.  Therefore, we know that $\zeta_{K,b^K}\in\cV_\zeta$.

\textbf{Part 2.} Now we show that for any $\zeta\in\cV_\zeta$, we have $\xi(\zeta)\in\cV_\xi$. Note that $\xi(\zeta)$ is given by
\#\label{eq:expl_xi}
& \xi^1(\zeta) = \zeta^1 - J(K, b^K), \notag\\
& \xi^2(\zeta) = \EE_{\pi_{K,b^K}}\bigl[\psi(x,u)\bigr] \zeta^1+ \Theta_{K,b^K} \zeta^2  - \EE_{\pi_{K,b^K}}\bigl[ c(x,u) \psi(x,u) \bigr]. 
\#
Then we have 
\#\label{eq:xi1}
\bigl|\xi^1(\zeta)\bigr| = \bigl|\zeta^1 - J(K, b^K)\bigr|\leq J_0
\#
and also 
\#\label{eq:xi2_1}
\bigl\|\xi^2(\zeta)  \bigr\|_2\leq \underbrace{\Bigl\|  \EE_{\pi_{K,b^K}}\bigl[\psi(x,u)\bigr] \zeta^1 \Bigr\|_2}_{B_1} + \underbrace{\|\Theta_{K,b^K}\|_*\cdot \|\zeta^2\|_2}_{B_2} + \underbrace{\Bigl\|\EE_{\pi_{K,b^K}}\bigl[ c(x,u) \psi(x,u) \bigr]\Bigr\|_2}_{B_3}. 
\#
Note that we can upper bound $B_1$ in the sequel
\#\label{eq:bound_B1}
B_1 \leq J_0\cdot  \Bigl\|  \EE_{\pi_{K,b^K}}\bigl[\psi(x,u)\bigr]  \Bigr\|_2 \leq J_0\cdot \|\Sigma_z\|_\F,
\#
where $\Sigma_z$ is given in \eqref{eq:sigma_z_factor}. Also, by Proposition \ref{prop:invert_theta}, we can bound $B_2$ in the following way
\#\label{eq:bound_B2}
B_2 \leq 4 ( 1 + \|K\|_\F^2 )^3\cdot \|\Phi_K^x\|_*^2 \cdot (M_{\zeta,1} + M_{\zeta,2})\cdot \bigl[ 1-\rho(A-BK) \bigr]^{-1}. 
\#
As for the term $B_3$ in \eqref{eq:xi2_1},  we utilize the following lemma to provide an upper bound. 

\begin{lemma}\label{lemma:form_c_psi}
The vector $\EE_{\pi_{K, b^K}}[c(x,u)\psi(x,u)]$ can be written in thee following way
\$
\EE_{\pi_{K, b^K}}[c(x,u)\psi(x,u)]& = \begin{pmatrix}
2\svec\bigl[ \Sigma_z \diag(Q,R)\Sigma_z + \la \Sigma_z, \diag(Q,R)\ra \Sigma_z \bigr]\\
\Sigma_z\begin{pmatrix}
2Q\mu_{K,b}^x\\
2R\mu_{K,b}^u
\end{pmatrix}
\end{pmatrix}\notag\\
&\qquad + ((\mu_{K,b}^x)^\top Q\mu_{K,b}^x + (\mu_{K,b}^u)^\top R\mu_{K,b}^u + \mu^\top \overline Q\mu)\begin{pmatrix}
\svec(\Sigma_z)\\
\mathbf{0}_{k+d}
\end{pmatrix}.
\$
Here the matrix $\Sigma_z$ is given in \eqref{eq:sigma_z_factor}. 
\end{lemma}
\begin{proof}
Please see \S\ref{proof:lemma:form_c_psi} for detailed proof. 
\end{proof}

From the above Lemma \ref{lemma:form_c_psi} and \eqref{eq:bound_mu_P}, we obtain the upper bound for $B_3$
\#\label{eq:bound_B3}
B_3\leq 3 \bigl[ \|Q\|_\F + \|R\|_\F  + J_0\|Q\|_* / \sigma_{\min}(Q) + J_0\|R\|_* / \sigma_{\min}(R)   \bigr] \cdot \|\Sigma_z\|_*^2. 
\#
Moreover, by the definition of $\Sigma_z$ in \eqref{eq:sigma_z_factor}, combining the triangular inequality, we have the following bounds for the Frobenius norm and spectral norm of $\Sigma_z$, respectively:
\#\label{eq:sigmaz_bound}
\|\Sigma_z\|_\F \leq 2(d + \|K\|_\F^2)\cdot \|\Phi_K^x\|_*, \qquad \|\Sigma_z\|_* \leq 2(1 + \|K\|_\F^2)\cdot \|\Phi_K^x\|_*. 
\#
Also, by similar techniques we used in deriving \eqref{eq:bound_mu_P}, we have
\$
J_0 \geq J(K,b^K)\geq \tr\bigl[ (Q + K^\top RK) \Phi_K^x \bigr] \geq \|\Phi_K^x\|_* \cdot \sigma_{\min}(Q),
\$
which gives the upper bound for $\Phi_K^x$ as follows
\#\label{eq:bound_phix}
\|\Phi_K^x\|_* \leq J_0 / \sigma_{\min}(Q). 
\#
Therefore, combining \eqref{eq:xi2_1}, \eqref{eq:bound_B1}, \eqref{eq:bound_B2}, \eqref{eq:bound_B3}, \eqref{eq:sigmaz_bound} and \eqref{eq:bound_phix}, we know that 
\#\label{eq:xi2}
\bigl\|\xi^2(\zeta)  \bigr\|_2\leq C\cdot (M_{\zeta,1} + M_{\zeta,2}) \cdot J_0^2/\sigma^2_{\min}(Q) \cdot \bigl( 1 + \|K\|_\F^2 \bigr)^3\cdot \bigl[ 1-\rho(A-BK) \bigr]^{-1}. 
\#
By \eqref{eq:xi1} and \eqref{eq:xi2}, we know that $\xi(\zeta)\in\cV_\xi$ for any $\zeta\in\cV_\zeta$. From this, we conclude the lemma.

\end{proof}

\subsection{Proof of Lemma \ref{lemma:form_c_psi}}\label{proof:lemma:form_c_psi}
\begin{proof}
First, note that the cost function $c(x,u)$ can be written in the following way
\$
c(x,u) = \psi(x,u)^\top \begin{pmatrix}
\svec\bigl[ \diag(Q,R) \bigr]\\
2Q\mu_{K,b}^x\\
2R\mu_{K,b}^u
\end{pmatrix} + ((\mu_{K,b}^x)^\top Q\mu_{K,b}^x + (\mu_{K,b}^u)^\top R\mu_{K,b}^u + \mu^\top \overline Q\mu). 
\$
For any test matrix $V$ and vectors $v_x$, $v_u$, we proceed by the following calculations
\#\label{eq:d1pd2}
& \EE_{\pi_{K,b^K}} \bigl[ c(x,u)\psi(x,u) \bigr]^\top \begin{pmatrix}
\svec(V)\\
v_x\\
v_u
\end{pmatrix}\notag \\
&\qquad = \EE_{\pi_{K, b^K}}\vast\{  \psi(x,u)^\top\begin{pmatrix}
\svec\bigl[\diag(Q,R) \bigr]\\
2Q\mu_{K,b}^x\\
2R\mu_{K,b}^u
\end{pmatrix} \psi(x,u)^\top \begin{pmatrix}
\svec(V)\\
v_x\\
v_u
\end{pmatrix}  \vast\}\notag \\
&\qquad\qquad+ \EE_{\pi_{K, b^K}}\vast\{\psi(x,u)^\top ((\mu_{K,b}^x)^\top Q\mu_{K,b}^x + (\mu_{K,b}^u)^\top R\mu_{K,b}^u + \mu^\top \overline Q\mu)  \begin{pmatrix}
\svec(V)\\
v_x\\
v_u
\end{pmatrix}\vast\} =: D_1 + D_2. 
\#
In the sequel, we calculate $D_1$ and $D_2$ respectively. 

\textbf{Calculation of $D_1$. } Note that from the definition of $\psi(x,u)$ in \eqref{eq:def_feature}, we can calculate $D_1$ as follows
\#\label{eq:D1_1}
D_1&  = \EE_{\pi_{K, b^K}} \vast\{\Biggl [ (z-\mu_z)^\top \diag(Q,R) (z-\mu_z)  +(z-\mu_z)^\top \begin{pmatrix}
2Q\mu_{K,b}^x\\
2R\mu_{K,b}^u
\end{pmatrix} \Biggr ]\notag\\
&\qquad\qquad \cdot  \Biggl [ (z-\mu_z)^\top V (z-\mu_z)  +(z-\mu_z)^\top \begin{pmatrix}
v_x\\
v_u
\end{pmatrix} \Biggr ]   \vast\}\notag\\
& = \EE_{\pi_{K, b^K}} \bigl [ (z-\mu_z)^\top \diag(Q,R) (z-\mu_z) \cdot (z-\mu_z)^\top V (z-\mu_z) \bigr]  \notag\\
& \qquad + \EE_{\pi_{K, b^K}} \Biggl[ \begin{pmatrix}
2Q\mu_{K,b}^x\\
2R\mu_{K,b}^u
\end{pmatrix}^\top (z-\mu_z)  (z-\mu_z)^\top \begin{pmatrix}
v_x\\
v_u
\end{pmatrix}  \Biggr]. 
\#
Here $z = (x^\top, u^\top)^\top$ and $\mu_z = \EE_{\pi_{K,b^K}}(z)$.  For the first on the RHS of \eqref{eq:D1_1}, note that $z-\mu_z$ is actually a centralized Gaussian, whose covariance matrix $\Sigma_z$ is given in \eqref{eq:sigma_z_factor}, therefore, by Lemma \ref{lemma:magnus}, we obtain that
\$
& \EE_{\pi_{K, b^K}} \bigl [ (z-\mu_z)^\top \diag(Q,R) (z-\mu_z) \cdot (z-\mu_z)^\top V (z-\mu_z) \bigr]\\
& \qquad = 2\bigl\la \Sigma_z \diag(Q,R) \Sigma_z, V\bigr\ra + \bigl\la \Sigma_z, \diag(Q, R)\bigr \ra \cdot \la \Sigma_z, V\ra\\
& \qquad = \svec\Bigl[ 2 \Sigma_z \diag(Q,R)\Sigma_z +  \bigl\la \Sigma_z, \diag(Q, R)\bigr \ra \cdot  \Sigma_z  \Bigr]^\top \svec(V). 
\$
Moreover, the second term on the RHS of \eqref{eq:D1_1} can be calculated as follows
\$
 \EE_{\pi_{K, b^K}} \Biggl[ \begin{pmatrix}
2Q\mu_{K,b}^x\\
2R\mu_{K,b}^u
\end{pmatrix}^\top (z-\mu_z)  (z-\mu_z)^\top \begin{pmatrix}
v_x\\
v_u
\end{pmatrix}  \Biggr] = \Biggl[\Sigma_z \begin{pmatrix}
2Q\mu_{K,b}^x\\
2R\mu_{K,b}^u
\end{pmatrix}\Biggr]^\top \begin{pmatrix}
v_x\\
v_u
\end{pmatrix}. 
\$
Combining the above two equations and \eqref{eq:D1_1}, we obtain that 
\#\label{eq:D1}
D_1 = \begin{pmatrix}
2\svec\bigl[ \Sigma_z \diag(Q,R)\Sigma_z + \la \Sigma_z, \diag(Q,R)\ra \Sigma_z \bigr]\\
\Sigma_z\begin{pmatrix}
2Q\mu_{K,b}^x\\
2R\mu_{K,b}^u
\end{pmatrix}
\end{pmatrix}^\top \begin{pmatrix}
\svec(V)\\
v_x\\
v_u
\end{pmatrix}. 
\#

\textbf{Calculation of $D_2$: } By the definition of the feature vector $\psi(x,u)$ in \eqref{eq:def_feature}, we know that 
\#\label{eq:D2}
D_2 =  ((\mu_{K,b}^x)^\top Q\mu_{K,b}^x + (\mu_{K,b}^u)^\top R\mu_{K,b}^u + \mu^\top \overline Q\mu) \begin{pmatrix}
\svec(\Sigma_z)\\
\mathbf{0}_{k+d}
\end{pmatrix}^\top \begin{pmatrix}
\svec(V)\\
v_x\\
v_u
\end{pmatrix}. 
\#

Now, combining \eqref{eq:d1pd2}, \eqref{eq:D1} and \eqref{eq:D2}, we conclude the lemma. 
\end{proof}

\subsection{Proof of Lemma \ref{lemma:bound_tilde_F}}\label{proof:lemma:bound_tilde_F}
\begin{proof}
We continue using the notations mentioned before.  
\textbf{Part 1.} First we characterize $|F(\zeta, \xi) - \hat F(\zeta, \xi)|$.  Note that by algebra, we have
\#\label{eq:diff_hat_F}
\bigl|F(\zeta, \xi) - \hat F(\zeta, \xi)\bigr| & = \biggl|  \Bigl\{ \EE(\psi - \hat\psi)\zeta^1 + \EE\bigl[ (\psi - \psi')\psi^\top - (\hat \psi - \hat\psi')\hat\psi^\top \bigr] \zeta^2 - \EE\bigl[ c(\psi - \hat\psi) \bigr]  \Bigr\}^\top \xi^2   \biggr|\notag\\
& \leq \EE\bigl(\|\psi - \hat\psi\|_2\bigr) \cdot \Big[  |\zeta^1|  +   \EE\bigl(   \| \psi - \psi' \|_2 + 2\|\hat\psi\|_2    \bigr)   \| \zeta^2 \|_2   + \EE( c)     \Bigr]\cdot \|\xi^2\|_2,
\#
where the expectation is taken over the trajectory generated by the policy $\pi_{K, b^K}$.   Note that with probability at least $1-(T^\mu)^{-6}$, the term $\EE(   \| \psi - \psi' \|_2 + 2\|\hat\psi\|_2 )$ can be bounded using a polynomial $\poly( \|\Phi_K^x\|_*, \|K\|_\F, \|b^K\|_2, \|\mu\|_2 )$. Also, the term $\EE(c)$ can also be bounded by a polynomial $\poly( \|\Phi_K^x\|_*, \|K\|_\F, \|b^K\|_2, \|\mu\|_2 )$. Therefore, combining Assumption \ref{assum:proj} and \eqref{eq:diff_hat_F}, with probability at least $1-(T^\mu)^{-6}$, we obtain that
\#\label{eq:diff_hat_F2}
\bigl|F(\zeta, \xi) - \hat F(\zeta, \xi)\bigr| \leq \EE\bigl(\|\psi - \hat\psi\|_2\bigr)\cdot \poly\bigl( \|\Phi_K^x\|_*, \|K\|_\F, \|b^K\|_2, \|\mu\|_2 \bigr). 
\#
Moreover, we can upper bound the term $\|\psi(x,u) - \hat\psi(x,u)\|_2$ for any $x$ and $u$ as follows
\#\label{eq:error_psi}
\|\psi(x,u) - \hat\psi(x,u)\|_2^2&  = \|\hat \mu_z - \mu_z\|_2^2 + \bigl\|   z(\hat\mu_z - \mu_z)^\top + (\hat\mu_z - \mu_z)z^\top  \bigr\|_\F^2 + \| \mu_z\mu_z^\top - \hat\mu_z \hat\mu_z^\top \|_\F^2\notag\\
& \leq \poly\bigl( \|\Phi_K^x\|_*, \|K\|_\F, \|b^K\|_2, \|\mu\|_2 \bigr) \cdot \| \hat\mu_z - \mu_z \|_2^2,
\#
and furthermore, by Lemma \ref{lemma:dist_hat_muz}, we know that 
\#\label{eq:error_muz}
\| \hat\mu_z - \mu_z \|_2 \leq \frac{\log T^\mu}{T^\mu}\cdot \poly\bigl( \|\Phi_K^x\|_*, \|K\|_\F, \|b^K\|_2, \|\mu\|_2 \bigr),
\#
holds with probability at least $1 - (T^\mu)^{-6}$.  Therefore, combining \eqref{eq:diff_hat_F2}, \eqref{eq:error_psi} and \eqref{eq:error_muz}, we know that it holds that
\#\label{eq:bound_F_hatF}
\bigl|F(\zeta, \xi) - \hat F(\zeta, \xi)\bigr| \leq   \frac{\log T^\mu}{T^\mu}\cdot \poly\bigl( \|\Phi_K^x\|_*, \|K\|_\F, \|b^K\|_2, \|\mu\|_2 \bigr)
\#
with probability at least $1 - (T^\mu)^{-6}$. 

\textbf{Part 2.} We now characterize $|\hat F(\zeta, \xi) - \tilde F(\zeta, \xi)|$ in the sequel.  By definitions, we have
\#\label{eq:diff_tilde_hat_F}
& \bigl|\tilde F(\zeta, \xi) - \hat F(\zeta, \xi)\bigr|\notag\\
&\qquad  =   \biggl|  \Bigl\{ \EE(\tilde \psi - \hat\psi)\zeta^1 + \EE\bigl[ (\tilde \psi - \tilde \psi')\tilde \psi^\top - (\hat \psi -  \hat\psi')\hat\psi^\top \bigr] \zeta^2 - \EE( \tilde c\tilde \psi - \hat c \hat \psi )  \Bigr\}^\top \xi^2  + \EE(\hat c - \tilde c)\xi^1  \biggr|\notag\\
& \qquad \leq  \biggl|  \Bigl\{ \EE(\hat\psi) \zeta^1 + \EE ( \hat \psi \hat\psi^\top )  \zeta^2 - \EE( \hat c \hat \psi )    \Bigr\}^\top \xi^2  + \EE(\hat c) \xi^1  \biggr|\cdot \ind_{\cE^c} + \Bigl|  \bigl[\EE(\hat \psi'\hat \psi^\top)\zeta^2\bigr]^\top \xi^2  \Bigr|\cdot \ind_{(\cE'\cap\cE)^c},
\#
where $\cE'$ is an event defined as 
\$
\cE' = \biggl(\bigcap_{t \in[T]}\Bigl\{   \bigl |  \| z_t' -\mu_z + 1/T^\mu\cdot \mu_{T^\mu}  \|_2^2 - \tr(\tilde \Sigma_z)    \bigr|   \leq    C_1\cdot \log T\cdot \|\tilde \Sigma_z\|_*   \Bigr\} \biggr) \bigcap  \cE_2,
\$
which, again by Lemma \ref{lemma:hwineq}, also satisfies that $\PP(\cE')\geq 1 - T^{-5} - (T^\mu)^{-6}$.  Moreover, by a similar argument as before, we can upper bound the two absolute values on the RHS of \eqref{eq:diff_tilde_hat_F}, which gives that
\#\label{eq:bound_tilde_hat_F}
\bigl|\tilde F(\zeta, \xi) - \hat F(\zeta, \xi)\bigr| \leq \frac{1}{2T} + \frac{1}{2T^\mu}
\#
for a sufficiently large $T$ and $T^\mu$. Therefore, combining \eqref{eq:bound_F_hatF} and \eqref{eq:bound_tilde_hat_F}, by using triangular inequality, and the fact that the term $\|\Phi_K^x\|_*$ can be bounded using $\|K\|_\F$, we finish the proof of this lemma. 
\end{proof}

\subsection{Proof of Lemma \ref{lemma:cost_diff}}\label{proof:lemma:cost_diff}
\begin{proof}
Note that by the fact that $P_{K_2}$ satisfies the Bellman equation in \eqref{eq:bellman}, we have
\$
 y^\top P_{K_2} y = \sum_{t\geq 0} y^\top \bigl[ (A-BK_2)^t  \bigr]^\top (Q + K_2^\top RK_2) (A-BK_2)^t y. 
\$
By the dynamics $y_{t + 1} = (A-BK_2)y_t$, we know that $y_t = (A-BK_2)^t y$; therefore, it holds that
\$
 y^\top P_{K_2} y = \sum_{t\geq 0} y_t^\top (Q + K_2^\top RK_2) y_t =  \sum_{t\geq 0} (y_t^\top Q y_t + y_t^\top K_2^\top RK_2 y_t).
\$
Then by telescoping, we have the follows
\#\label{eq:telesum}
 y^\top P_{K_2} y -  y^\top P_{K_1} y =  \sum_{t\geq 0} (y_t^\top Q y_t + y_t^\top K_2^\top RK_2 y_t  +  y_{t+1}^\top P_{K_1} y_{t + 1}-  y_{t}^\top P_{K_1} y_{t } ). 
\#
Moreover, note that for any $t\geq 0$, we have
\#\label{eq:telesum2}
& y_t^\top Q y_t + y_t^\top K_2^\top RK_2 y_t  +  y_{t+1}^\top P_{K_1} y_{t + 1}-  y_{t}^\top P_{K_1} y_{t }\notag\\
& \qquad = y_t^\top \bigl[ Q + (K_2 - K_1 + K_1)^\top R (K_2 - K_1 + K_1) \bigr]y_t\notag\\
&\qquad\qquad +  y_t^\top \bigl[ A-BK_1 - B(K_2 - K_1) \bigr]^\top P_{K_1} \bigl[ A-BK_1 - B(K_2 - K_1) \bigr] y_t - y_t^\top P_{K_1}y_t\notag\\
& \qquad = 2y_t^\top  (K_2 - K_1)^\top \bigl[ (R + B^\top P_{K_1}B)K_1 - B^\top P_{K_1}A \bigr] y_t + y_t^\top (K_2 - K_1)^\top (R + B^\top P_{K_1}B)(K_2 - K_1) y_t\notag\\
& \qquad = 2y_t^\top  (K_2 - K_1)^\top ( \Upsilon_{K_1}^{22} K_1 - \Upsilon_{K_1}^{21} ) y_t + y_t^\top (K_2 - K_1)^\top \Upsilon_{K_1}^{22} (K_2 - K_1) y_t. 
\#
Combining \eqref{eq:telesum} and \eqref{eq:telesum2}, we finish the proof. 
\end{proof}

\subsection{Proof of Lemma \ref{lemma:grad_dom}}\label{proof:lemma:grad_dom}
\begin{proof}
\textbf{Upper Bound. }    From the definition of $J_1(K)$ in \eqref{eq:a2}, we have
\#\label{eq:JJ_diff1}
J_1(K) - J_1(K^*)&  = \tr( P_K\Psi_\epsilon - P_{K^*}\Psi_\epsilon ) = \EE_{y\sim \mathcal N(0, \Psi_\epsilon)} (y^\top P_K y - y^\top P_{K^*} y )\notag\\
& =  -\EE_{y_0\sim\mathcal N(0,\Psi_\epsilon)}\Biggl[ \sum_{t\geq 0} D_{K, K^*} (y_t) \Biggr],
\#
where in the last equality, we apply Lemma \ref{lemma:cost_diff} and $\{y_t\}_{t\geq0}$ follows the dynamics $y_{t+ 1} = (A- BK^*)y_t$.  Further,  we can write $D_{K, K^*}(y)$ in the following way
\#\label{eq:bound_D1}
D_{K, K^*}(y)& = 2y^\top (K^* - K)(\Upsilon_K^{22} K  - \Upsilon_K^{21}) y + y^\top (K^* - K)^\top\Upsilon_K^{22} (K^* - K)x\notag\\
& = y^\top \bigl[ K^* - K + (\Upsilon_K^{22})^{-1}  (\Upsilon_K^{22} K  - \Upsilon_K^{21}) \bigr]^\top \Upsilon_K^{22} \bigl[ K^* - K + (\Upsilon_K^{22})^{-1}  (\Upsilon_K^{22} K  - \Upsilon_K^{21}) \bigr] y  \notag\\
&\qquad\qquad -y^\top (\Upsilon_K^{22} K  - \Upsilon_K^{21})^\top (\Upsilon_{K}^{22})^{-1}(\Upsilon_K^{22} K  - \Upsilon_K^{21})y. 
\#
Note that the first term on the RHS of \eqref{eq:bound_D1} is positive, due to the fact that it is a quadratic form of a positive definite matrix, we therefore can lower bound $D_{K, K^*}(y)$ as follows
\#\label{eq:bound_D}
D_{K, K^*}(y) \geq -y^\top (\Upsilon_K^{22} K  - \Upsilon_K^{21})^\top (\Upsilon_{K}^{22})^{-1}(\Upsilon_K^{22} K  - \Upsilon_K^{21})y. 
\#
Therefore, combining \eqref{eq:JJ_diff1} and \eqref{eq:bound_D}, it holds that
\#\label{eq:JJ_diff2}
J_1(K) - J_1(K^*) & \leq   \Biggl\|  \EE_{y_0\sim\mathcal N(0, \Psi_\epsilon)}  \Biggl[ \sum_{t\geq 0}  y_t y_t^\top\Biggr] \Biggr \|_*   \cdot  \tr\bigl[(\Upsilon_K^{22} K  - \Upsilon_K^{21})^\top (\Upsilon_{K}^{22})^{-1}(\Upsilon_K^{22} K  - \Upsilon_K^{21})\bigr]\notag\\
& = \| \Phi^x_{K^*} \|_*\cdot \tr\bigl[(\Upsilon_K^{22} K  - \Upsilon_K^{21})^\top (\Upsilon_{K}^{22})^{-1}(\Upsilon_K^{22} K  - \Upsilon_K^{21})\bigr]\notag\\
& \leq  \bigl\|(\Upsilon_{K}^{22})^{-1}\bigr\|_* \cdot   \| \Phi^x_{K^*} \|_*\cdot \tr\bigl[(\Upsilon_K^{22} K  - \Upsilon_K^{21})^\top (\Upsilon_K^{22} K  - \Upsilon_K^{21})\bigr]\notag\\
& \leq \sigma_{\min}^{-1}(R) \cdot   \| \Phi^x_{K^*} \|_*\cdot \tr\bigl[(\Upsilon_K^{22} K  - \Upsilon_K^{21})^\top (\Upsilon_K^{22} K  - \Upsilon_K^{21})\bigr],
\#
where the second line comes from direct computation, while the last line comes from the fact that $\Upsilon_{K}^{22} = R + B^\top KP_ B\preceq R$.  This complete the proof of the upper bound. 

\textbf{Lower Bound. }  Note that for any policy parameter $\tilde K$, the following inequality holds:
\#\label{eq:JJ_diff3}
J(K) - J(K^*)\geq J(K) - J(\tilde K ) = -\EE_{y_0\sim\mathcal N(0,\Psi_\epsilon)}\Biggl[ \sum_{t\geq 0} D_{K, \tilde K} (y_t) \Biggr],
\#
where $\{y_t\}_{t\geq0}$ follows the dynamics $y_{t+ 1} = (A- B\tilde K)y_t$. 
Therefore, by choosing $\tilde K = K - (\Upsilon_K^{22})^{-1}  (\Upsilon_K^{22} K  - \Upsilon_K^{21})$, by a similar calculation as shown in \eqref{eq:bound_D1}, the function $D_{K, \tilde K}(y)$ takes the form
\#\label{eq:form_D_tilde}
D_{K, \tilde K}(y)& = -y^\top (\Upsilon_K^{22} K  - \Upsilon_K^{21})^\top (\Upsilon_{K}^{22})^{-1}(\Upsilon_K^{22} K  - \Upsilon_K^{21})y. 
\#
By combining \eqref{eq:JJ_diff3} and \eqref{eq:form_D_tilde}, we obtain a lower bound as follows
\$
J(K) - J(K^*)& \geq \tr\bigl[ \Phi^x_{\tilde K}  (\Upsilon_K^{22} K  - \Upsilon_K^{21})^\top (\Upsilon_{K}^{22})^{-1}(\Upsilon_K^{22} K  - \Upsilon_K^{21})  \bigr]\\
& \geq \sigma_{\min}(\Psi_\epsilon) \cdot \| \Upsilon_{K}^{22} \|_*^{-1}\cdot \tr\bigl[ (\Upsilon_K^{22} K  - \Upsilon_K^{21})^\top (\Upsilon_K^{22} K  - \Upsilon_K^{21}) \bigr]. 
\$
Here in the last line, we use the fact that $\Phi_{\tilde K}^x\succeq \Psi_\epsilon$.  This finishes the proof of the lower bound.  
\end{proof}

\subsection{Proof of Lemma \ref{lemma:error_bound_tilde_J}}\label{proof:lemma:error_bound_tilde_J}
\begin{proof}
By direct calculation and Proposition \ref{prop:cost_form}, we have
\#\label{eq:312diff1}
\bigl|J_1(\tilde  K_{n+1}) - J_1( K_{n+1})\bigr| =  \tr\bigl[ (P_{\tilde K_{n+1}} - P_{ K_{n+1}} ) \Psi_\epsilon \bigr]\leq \|P_{\tilde K_{n+1}} - P_{ K_{n+1}}\|_*\cdot \|\Psi_\epsilon\|_\F. 
\#
The following lemma helps establish the upper bound of the term $\|P_{\tilde K_{n+1}} - P_{ K_{n+1}}\|_*$.  

\begin{lemma}\label{lemma:perturb}
Suppose that the policy parameters $K$ and $\tilde K$ satisfy that
\#\label{eq:perturbK}
\| \tilde K - K \|_*\cdot \bigl( \|A-BK\|_* +1 \bigr) \cdot \| \Phi^x_K \|_*  \leq \sigma_{\min}(\Psi_\omega)/4\cdot \|B\|_*^{-1}, 
\#
then it holds that
\#\label{eq:perturbPK}
\| P_{\tilde K} - P_K \|_* & \leq 6\cdot \sigma_{\min}^{-1} (\Psi_\omega)\cdot \|\Phi_K^x\|_* \cdot \|K\|_*\cdot \|R\|_*\cdot \|\tilde   K- K\|_*  \\
&\qquad \cdot \bigl( \|B\|_*\cdot \|K\|_*)\cdot \|A-BK\|_* + \|B\|_*\cdot\|K\|_* + 1 \bigr). 
\#
\end{lemma}
\begin{proof}
{\red See somewhere}
\end{proof}

To use the above Lemma \ref{lemma:perturb}, we only need to verify that the perturbation $\|\tilde K_{n+1} - K_{n+1}\|_*$ satisfies the condition \eqref{eq:perturbK}. Note that from \eqref{eq:ac_update_Kn} and \eqref{eq:tilde_update_Kn}, we have
\#\label{eq:veridiff1}
& \| \tilde K_{n+1} - K_{n+1} \|_* \cdot \bigl( \|A-B\tilde K_{n+1}\|_* +1 \bigr) \cdot \| \Phi^x_{\tilde K_{n+1}} \|_*  \notag\\
&\qquad\leq \gamma\cdot \|\hat \Upsilon_{K_n} - \Upsilon_{K_n}\|_\F \cdot \bigl( 1 + \| K_n \|_* \bigr)\cdot \bigl( \|A-B\tilde K_{n+1}\|_* +1 \bigr) \cdot \| \Phi^x_{\tilde K_{n+1}} \|_*. 
\#
Now we proceed to upper bound each term on the RHS of \eqref{eq:veridiff1}.  For the term $\|A-B\tilde K_{n+1}\|_*$, we have
\#\label{eq:veribd1}
\|A-B\tilde K_{n+1}\|_*& \leq \|A-BK_n\|_* + \gamma\cdot \| B \|_*\cdot \|\Upsilon_{K_n}^{22}K_n - \Upsilon_{K_n}^{21}\|_*\notag\\
& \leq \|A-BK_n\|_* + \gamma\cdot \| B \|_*\cdot \|\Upsilon_{K_n}\|_*\cdot \bigl(1 + \|K_n\|_* \bigr).
\#
And from the form of $\Upsilon_{K_n}$ proposed in \eqref{eq:def_upsilon}, we can upper bound $\|\Upsilon_{K_n}\|_*$ as 
\#\label{eq:veribd2}
\|\Upsilon_{K_n}\|_* & \leq \|Q\|_* + \|R\|_* + \bigl( \|A\|_\F + \|B\|_\F \bigr)^2\cdot \|P_{K_n}\|_*\notag\\
&\leq \|Q\|_* + \|R\|_* + \bigl( \|A\|_\F + \|B\|_\F \bigr)^2\cdot J_1(K_0) \cdot \sigma_{\min}^{-1}(\Psi_\epsilon), 
\#
where the last line comes from the fact that $\|P_{K_n}\|_* \leq J_1(K_n)\cdot \sigma_{\min}^{-1}(\Psi_\epsilon)\leq J_1(K_0)\cdot \sigma_{\min}^{-1}(\Psi_\epsilon)$.   As for the term $ \| \Phi^x_{\tilde K_{n+1}} \|_*$ in \eqref{eq:veridiff1}, we can upper bound it as
\#\label{eq:veribd3}
 \| \Phi^x_{\tilde K_{n+1}} \|_* \leq J_1(\tilde K_{n+1})\cdot \sigma_{\min}^{-1}(Q) \leq J_1(K_0) \cdot \sigma_{\min}^{-1}(Q). 
\#
Therefore, combining \eqref{eq:veridiff1}, \eqref{eq:veribd1}, \eqref{eq:veribd2} and \eqref{eq:veribd3}, we know that 
\#\label{eq:veridiff2}
& \| \tilde K_{n+1} - K_{n+1} \|_* \cdot \bigl( \|A-B\tilde K_{n+1}\|_* +1 \bigr) \cdot \| \Phi^x_{\tilde K_{n+1}} \|_*  \notag\\
&\qquad \leq \poly_1\bigl( \|K_n\|_*, J_1(K_0) \bigr) \cdot  \|\hat \Upsilon_{K_n} - \Upsilon_{K_n}\|_\F. 
\#
Also, by the above results, the RHS of \eqref{eq:perturbPK} can be bounded as
\#\label{eq:perturbPK2}
& 6\cdot \sigma_{\min}^{-1} (\Psi_\omega)\cdot \|\Phi_{\tilde K_{n+1}}^x\|_* \cdot \|\tilde K_{n+1}\|_*\cdot \|R\|_*\cdot \|\tilde K_{n+1}-  K_{n+1}\|_*  \notag\\
&\qquad\qquad\cdot \bigl( \|B\|_*\cdot \|\tilde K_{n+1}\|_*)\cdot \|A-B\tilde K_{n+1}\|_* + \|B\|_*\cdot\|\tilde K_{n+1}\|_* + 1 \bigr)\notag\\
&\qquad\leq \poly_2\bigl(\|K_n\|_*, J_1(K_0)\bigr)\cdot  \|\hat \Upsilon_{K_n} - \Upsilon_{K_n}\|_\F. 
\# 
Note that from the policy evaluation theorem \ref{thm:pe}, we know that with probability at least $1-T^{-4} - (T^\mu)^{-6}$, it holds that
\#\label{eq:res_from_pe}
\|\hat\Upsilon_{K_n} - \Upsilon_{K_n}\|_\F &  \leq  \frac{\poly_3 \bigl(  \|K_n\|_\F, \|\mu\|_2  \bigr) }{ \lambda_{K_n}\cdot\sqrt{ \log(1/\rho)} }\cdot\frac{\log^3 T_n}{T_n^{1/4}} \notag\\
&\qquad + \frac{\poly_4 \bigl( \|K_n\|_\F, \|b^{K_n}\|_2, \|\mu\|_2 \bigr)}{\lambda_{K_n}}\cdot \frac{\log^{1/2} T_n^\mu}{(T_n^\mu)^{1/2}}. 
\#
By choosing $T_n$ and $T_n^\mu$ such that
\$
& \frac{\poly_3 \bigl(  \|K_n\|_\F, \|\mu\|_2  \bigr) }{ \lambda_{K_n}\cdot\sqrt{ \log(1/\rho)} }\cdot\frac{\log^3 T_n}{T_n^{1/4}}  + \frac{\poly_4 \bigl( \|K_n\|_\F, \|b^{K_n}\|_2, \|\mu\|_2 \bigr)}{\lambda_{K_n}}\cdot \frac{\log^{1/2} T_n^\mu}{(T_n^\mu)^{1/2}}\notag\\
&\qquad \leq \max\biggl\{  \Bigl[\poly_1\bigl( \|K_n\|_*, J_1(K_0) \bigr)\Bigr]^{-1}\cdot \sigma_{\min}(\Psi_\omega)/4\cdot\|B\|_*^{-1} ,  \notag\\
&\qquad\qquad  \Bigl[\poly_2\bigl(\|K_n\|_*, J_1(K_0)\bigr)\Bigr]^{-1}\cdot \varepsilon/2\cdot \gamma\cdot \sigma_{\min}(\Psi_\epsilon)\cdot \sigma_{\min}(R)\cdot \|\Phi_{K^*}^x\|_*^{-1}\cdot \|\Psi_\epsilon\|_\F^{-1}   \biggr\}, 
\$
in other words, we can pick 
\$
& T_n\geq \poly_5 \bigl( \|K_n\|_\F, \|b^{K_n}\|_2, \|\mu\|_2 \bigr) \cdot \lambda_{K_n}^{-4} \cdot \bigl[1-\rho(A-BK_n)\bigr]^{-5}\cdot \varepsilon^{-5},\\
& T_n^\mu \geq \poly_6 \bigl( \|K_n\|_\F, \|b^{K_n}\|_2, \|\mu\|_2 \bigr) \cdot \lambda_{K_n}^{-2}\cdot \varepsilon^{-3}, 
\$
then we can see that the condition \eqref{eq:perturbK} holds with probability at least $1-\varepsilon^{10}$ for sufficiently small $\varepsilon > 0$. And then by applying Lemma \ref{lemma:perturb}, combining \eqref{eq:312diff1}, we can derive that
\#\label{eq:main_diff_J2}
\bigl|J_1(\tilde  K_{n+1}) - J_1( K_{n+1})\bigr| \leq \gamma\cdot \sigma_{\min}(\Psi_\epsilon)\cdot \sigma_{\min}(R)\cdot \|\Phi_{K^*}^x\|_*^{-1}\cdot  \varepsilon / 2
\#
holds with probability at least $1-\varepsilon^{10}$.  By this, we finish the proof of the lemma. 
\end{proof}

\subsection{Proof of Lemma \ref{lemma:convex_J2}}\label{proof:lemma:convex_J2}
\begin{proof}
By computing the Hessian matrix of $J_2(b;K)$ directly, we have
\$
 \nabla^2 J_2(b;K) = & B^\top (I-A+BK)^{-\top} (Q + K^\top RK)(I-A+BK)^{-1} B \notag\\
&\qquad - \bigl[RK(I-A+BK)^{-1}B + B^\top (I-A+BK)^{-\top}  K^\top R\bigr] + R\\
 = & \bigl[\sqrt{R}K(I-A+BK)^{-1}B - \sqrt{R}\bigr]^\top\bigl[\sqrt{R}K(I-A+BK)^{-1}B - \sqrt{R}\bigr] \notag\\
&\qquad + B^\top (I-A+BK)^{-\top} Q (I-A+BK)^{-1} B,
\$
which is a positive constant matrix. We assume that this matrix has minimum singular value $\nu_K > 0$. 
Moreover, note that $\nabla^2 J_2(b;K)$ can be upper bounded as
\$
\bigl\|\nabla^2 J_2(b;K)\bigr\|_* \leq \bigl[1-\rho(A-BK)\bigr]^{-2} \cdot \bigl(  \|B\|_*^2\cdot \|K\|_*^2\cdot \|R\|_* + \|B\|_*^2\cdot \|Q\|_* \bigr). 
\$
Therefore, we can see that the maximum singular value $\iota_K$ of $\nabla^2 J_2(b;K)$ satisfies that 
\$
\iota_K \leq \bigl[1-\rho(A-BK)\bigr]^{-2} \cdot \bigl(  \|B\|_*^2\cdot \|K\|_*^2\cdot \|R\|_* + \|B\|_*^2\cdot \|Q\|_* \bigr). 
\$
This finishes the proof. 
\end{proof}

\subsection{Proof of Lemma \ref{lemma:bound_tilde_J_2}}\label{proof:lemma:bound_tilde_J_2}
\begin{proof}
Note that by Lemma \ref{lemma:convex_J2}, we have
\#\label{eq:brute_force_bound0}
& J_2(b_{n+1}; K) - J_2(\tilde b_{n+1}; K)  \notag\\
&\qquad \leq \gamma^0\cdot  \nabla J_2(\tilde b_{n+1}; K)^\top \bigl[  \nabla J_2(b_n; K) - \hat\nabla J_2(b_n; K)  \bigr ] + (\gamma^0)^2\cdot \frac{\nu_K}{2}\bigl \|\nabla J_2(b_n; K) - \hat\nabla J_2(b_n; K)\bigr\|_2^2,\notag\\
& J_2(\tilde b_{n+1}; K) - J_2( b_{n+1}; K)  \notag\\
&\qquad \leq - \gamma^0\cdot  \nabla J_2(\tilde b_{n+1}; K)^\top \bigl[  \nabla J_2(b_n; K) - \hat\nabla J_2(b_n; K)  \bigr ] - (\gamma^0)^2\cdot\frac{\iota_K}{2} \bigl\|\nabla J_2(b_n; K) - \hat\nabla J_2(b_n; K)\bigr\|_2^2. 
\#
Moreover, we can upper bound $\| \nabla J_2(\tilde b_{n+1}; K)\|_2$ as follows
\#\label{eq:brute_force_bound}
\bigl\| \nabla J_2(\tilde b_{n+1}; K)\bigr\|_2 \leq \poly_1\bigl( \|K\|_\F, \|b_n\|_2,  \|\mu\|_2, J_0 \bigr)\cdot \bigl[1 -  \rho(A-BK) \bigr]^{-1}. 
\#
Combining \eqref{eq:brute_force_bound0}, \eqref{eq:brute_force_bound} and the fact that $\nu_K\leq \iota_K\leq [1-\rho(A-BK)]^{-2}\cdot \poly_2(\|K\|_*)$, we know that
\#\label{eq:diff_tildeb_b2}
&\bigl|J_2(b_{n+1}; K) - J_2(\tilde b_{n+1}; K)\bigr|\notag\\
 &\qquad  \leq \gamma^0\cdot  \poly_1\bigl( \|K\|_\F, \|b_n\|_2,  \|\mu\|_2, J_0 \bigr)\cdot \bigl\|  \nabla J_2(b_n; K) - \hat\nabla J_2(b_n; K)  \bigr \|_2 \cdot \bigl[1 -  \rho(A-BK) \bigr]^{-1}\notag\\
&\qquad\qquad  + (\gamma^0)^2 \cdot  \poly_2\bigl(\|K\|_*\bigr)  \cdot \bigl \|\nabla J_2(b_n; K) - \hat\nabla J_2(b_n; K)\bigr\|_2^2\cdot \bigl[1 -  \rho(A-BK) \bigr]^{-2}. 
\#
Note that from the definition of $\nabla J_2(b_n; K)$ and $\hat \nabla J_2(b_n; K)$, we have
\#\label{eq:bound_hat_grad1}
& \bigl \|  \nabla J_2(b_n; K)  - \hat \nabla J_2(b_n; K)  \bigr\|_2\notag\\
  &\qquad \leq \| \hat \Upsilon_K^{22} - \Upsilon_K^{22} \|_*\cdot \|K\|_*\cdot \|\hat\mu_{K, b_n}^x\|_2 + \|\Upsilon_K^{22} \|_*\cdot \|K\|_*\cdot \|\hat\mu_{K, b_n}^x - \mu_{K, b_n}^x\|_2 + \|\hat\Upsilon_K^{22} - \Upsilon_K^{22}\|_*\cdot \|b_n\|_2 \notag\\
& \qquad\qquad + \|\hat\Upsilon_K^{21} - \Upsilon_K^{21}\|_*\cdot \|\hat\mu_{K, b_n}^x \|_2 + \|\Upsilon_{K}^{21}\|_*\cdot \|\hat\mu_{K, b_n}^x - \mu_{K, b_n}^x  \|_2 + \|\hat q_{K, b_n} - q_{K, b_n}\|_2.
\#
From Theorem \ref{thm:pe} and Lemma \ref{lemma:dist_hat_muz}, combining the fact that $J_2(b_n; K) \leq J_2(b_0; K)$ and \eqref{eq:bound_mu_P}, we know that with probability at least $1 - T^{-4} - (T^\mu)^{-6}$, it holds that
\#\label{eq:bound_hat_grad2}
& \bigl \|  \nabla J_2(b_n; K)  - \hat \nabla J_2(b_n; K)  \bigr\|_2\notag\\
&\qquad \leq  \lambda_K^{-1}  \cdot  \poly_3\bigl( \|K\|_\F, \|b_n\|_2, \|\mu\|_2, J_2(K, b_0) \bigr)\cdot \biggl[ \frac{\log^3 T_n}{T_n^{1/4}(1-\rho)^{3/2}} +  \frac{\log^{1/2} T_n^\mu}{(T_n^\mu)^{1/2}}  \biggr]. 
\#
To show that \eqref{eq:lemma_bound_tilde} holds, we only need to pick $\gamma^0$, $T_n$ and $T_n^\mu$ such that
\$
& \gamma^0\cdot \poly_1\bigl( \|K\|_\F, \|b_n\|_2,  \|\mu\|_2, J_0 \bigr)\cdot \lambda_K^{-1}\cdot \poly_3\bigl( \|K\|_\F, \|b_n\|_2, \|\mu\|_2, J_2(K, b_0) \bigr)\\
&\qquad   \cdot  \biggl[ \frac{\log^3 T_n}{T_n^{1/4}(1-\rho)^{3/2}} +  \frac{\log^{1/2} T_n^\mu}{(T_n^\mu)^{1/2}}  \biggr]\cdot \bigl[1 -  \rho(A-BK) \bigr]^{-1} + (\gamma^0)^2\cdot \poly_2\bigl( \|K\|_* \bigr)  \cdot \lambda_K^{-1} \\
&\qquad\cdot \poly_3\bigl( \|K\|_\F, \|b_n\|_2, \|\mu\|_2, J_2(K, b_0) \bigr) \cdot  \biggl[ \frac{\log^6 T_n}{T_n^{1/2}(1-\rho)^{3}} +  \frac{\log T_n^\mu}{T_n^\mu}  \biggr]\cdot \bigl[1 -  \rho(A-BK) \bigr]^{-2}\\
& \quad \leq \nu_K\cdot \gamma^0\cdot \epsilon,
\$
in other words, we can pick
\$
& \gamma^0 \leq  1 - \rho(A-BK),\\
& T_n = \poly_4\bigl( \|K\|_\F, \|b_n\|_2, \|\mu\|_2, J_2(K, b_0) \bigr)\cdot \lambda_K^{-4}\cdot \nu_K^{-4}\cdot (1-\rho)^{-10}\cdot \varepsilon^{-5},\\
& T_n^\mu = \poly_5\bigl( \|K\|_\F, \|b_n\|_2, \|\mu\|_2, J_2(K, b_0) \bigr)\cdot \lambda_K^{-2}\cdot \nu_K^{-2}\cdot (1-\rho)^{-2}\cdot \varepsilon^{-2},
\$
then \eqref{eq:lemma_bound_tilde} holds with probability at least $1-\varepsilon^{10}$.  This finishes the proof. 
\end{proof}

\subsection{Proof of Lemma \ref{lemma:local_sc}}\label{proof:lemma:local_sc}
\begin{proof}
Note that from Lemma \ref{lemma:cost_diff}, it holds that
\$
J_1(K) - J_1(K^*)& = \EE\biggl\{  \sum_{t\geq 0}  \bigl[  2y_t^\top (K-K^*)(\Upsilon_{K^*}^{22}K^* - \Upsilon_{K^*}^{21})y_t + y_t^\top (K-K^*)^\top \Upsilon_{K^*}^{21}(K-K^*)y_t  \bigr]  \biggr\}\notag\\
& = \tr\bigl[ \Phi_{K}^x (K-K^*)^\top\Upsilon_{K^*}^{21}(K-K^*) \bigr]\notag\\
& \geq \|\Phi_K^x\|_*\cdot \| \Upsilon_{K^*}^{21} \|_* \cdot \tr\bigl[ (K-K^*)^\top(K-K^*) \bigr]\notag\\
& \geq \sigma_{\min}(\Psi_\epsilon)\cdot \sigma_{\min}(R) \cdot \|K-K^*\|_\F^2,
\$
where $\{y_t\}_{t\geq0}$ follows the dynamics $y_{t+1} = (A-BK)y_t$. Here in the second line, we use the fact that $\Upsilon_{K^*}^{22}K^* - \Upsilon_{K^*}^{21}$ is the natural gradient of $J_1(\cdot)$ evaluated at $K^*$, which implies that $\Upsilon_{K^*}^{22}K^* - \Upsilon_{K^*}^{21} = 0$; while in the last line, we use the fact that $\|\Phi_K^x\|_* \geq \sigma_{\min}(\Psi_\epsilon)$ and $\|\Upsilon_{K^*}^{21}\|_*\geq \sigma_{\min}(R)$.  This concludes the lemma.  
\end{proof}

\section{Auxiliary Results}

\begin{lemma}\label{lemma:magnus}
Assume that the random variable $w\sim\mathcal N(0,I)$, and let $U$ and $V$ be two symmetric matrices, then it holds that
\$
\EE[w^\top U w \cdot w^\top V w] = 2\tr(UV) + \tr(U)\cdot \tr(V). 
\$
\end{lemma}
\begin{proof}
Please see \cite{magnus1978moments, magnus1979expectation} for detail. 
\end{proof}

\begin{lemma}\label{lemma:alizadeh1998primal}
Let $M$, $N$ be commuting symmetric matrices, and let $\alpha_1, \ldots, \alpha_n$, $\beta_1, \ldots, \beta_n$ denote their eigenvalues with $v_1, \ldots, v_n$ a common basis of orthogonal eigenvectors. Then the $n(n+1)/2$ eigenvalues of $M\otimes_s N$ are given by $(\alpha_i\beta_j + \alpha_j\beta_i)/2$, where $1\leq i\leq j\leq n$. 
\end{lemma}
\begin{proof}
Please see Lemma 2 in \cite{alizadeh1998primal} for detail. 
\end{proof}

\begin{lemma}\label{lemma:hwineq}
For any integer $m>0$, let $A\in\RR^{m\times m}$ and $\eta\sim \mathcal N(0, I_m)$. Then, there exists some absolute constant $C>0$ such that for any $t\geq 0$, we have
\$
\PP\Bigl[ \bigl| \eta^\top A\eta - \EE(\eta^\top A\eta)   \bigr| > t \Bigr]  \leq 2\cdot \exp\Bigl[ -C\cdot \min\bigl(  t^2 \|A\|_\F^{-2}, ~t\|A\|_*^{-1}  \bigr) \Bigr]. 
\$
\end{lemma}
\begin{proof}
Please see \cite{rudelson2013hanson} for detail. 
\end{proof}
